# Supplementary material for: Multi-Agent Stochastic Bandits Robust to Adversarial Corruptions
Source: arXiv:2411.08167 source file (2024-11-12)
Supplement: Supplementary file 1 [file appendix-backup.tex]

\clearpage

\section{Single-Agent}
We define an event \(\mathcal{E}\) such as:
\begin{align}\label{eq:event-E_SA}
    \mathcal{E} \coloneqq \left\{\forall k\in \mathcal{K}, m \in \{1, 2, \dots, M\} : \left|r_{k}^m - \mu_k\right| \le 2\frac{C^m}{T^m} + \frac{\Delta_{k}^{m-1}}{16} \text{ and } \Tilde{n}_{k}^m \le {2 p^m_{k}T^m} \right\},
\end{align}
where \(C^m\) is the total corruption in epoch \(m\), and \(\Tilde{n}_{k}^m\) is the actual number of pulls of arm \(k\) in epoch \(m\).

% such that \(C = \sum_{\ell \in \mathcal{L}} \sum_{m = 1}^M C_\ell^m\)

\begin{lemma}\label{lem:4_SA}
    It holds that:
    \begin{align}
        \Pr[\mathcal{E}] \geq 1 - \delta.
    \end{align}
\end{lemma}


\begin{proof}
    % \(\beta \geq 4e^{-\frac{\lambda}{16L}}\), where \(L\) is the total number of agents.
    % For any fixed \(\ell \in \mathcal{L}\), \(k \in \mathcal{K}_{\ell}\), and \(m\) we have:
    \item
    \paragraph{Decomposing \(\pmb{r_{k}^m}\)}For this proof, we condition on all random variables before some fixed epoch \(m\), so that \(p^m_{k}\) is a deterministic quantity. At each step in this epoch, agent picks arm \(k\) with probability \(p_{k}^m\). Let \(Y_{k}^t\) be an indicator for arm \(k\) being pulled in step \(t\). Let \(R_{k}^t\) be the stochastic reward of arm \(k\) on step \(t\). and \(c^t_{k} \coloneqq \tilde{R}_{k}^t - R_{k}^t\) be the corruption added to arm \(k\) by the adversary in step \(t\). Note that \(c^t_{k}\) may depend on all the stochastic rewards up to (and including) round \(t\), and also on all previous choices of the algorithm (though not the choice at step \(t\)). Finally, we denote \(E^m\) to be the \(T^m\) timesteps in epoch \(m\), then we define a random variable \(r_{k}^m\) as follows:
    \begin{equation}
        r_{k}^m = \frac{1}{p_k^mT^m}\sum_{t \in E^m}Y_{k}^t\left(R_{k}^t + c_{k}^t\right).
    \end{equation}
    Let us break this sum into two:
    \begin{align*}
        A_{k}^m & = \sum_{t \in E^m}Y_{k}^tR_{k}^t  \\
        B_{k}^m & = \sum_{t \in E^m}Y_{k}^tc_{k}^t.
    \end{align*}

    \item
    \paragraph{Bounding the first and the second part} To \textbf{bound the first part}, we first note that:
    \begin{align*}
        \mathbb{E}\left[A_{k}^m\right] = T^m\left(p_{k}^m\mu_k\right),
    \end{align*}
    Therefore, according to the Chernoff-Hoeffding bound \cite{dubhashi2009concentration}, and because \(\mu_k \le 1\), for \(\beta \leq 1\) we have:
    \begin{align}
        \label{eqn:A2_SA}
        Pr\left[\left|\frac{A_{k}^m}{p_{k}^mT^m} - \mu_k\right| \geq \sqrt{\frac{3\ln{\frac{4}{\beta}}}{p_{k}^mT^m}}\right] \leq \frac{\beta}{2}.
    \end{align}


    Next, we aim to \textbf{bound the second part}. To this end, we define the sequence of r.v.s, \(\{X_{t}\}_{t\in[1,\dots, T]}\), where \(X_{t} = \left(Y_{k}^t - p_{k}^m\right)\cdot c_{k}^t\) for all \(t\). Then \(\{X_{t}\}_{t\in[1,\dots, T]}\) is a martingale sequence with respect to the filtration \(\{\mathcal{F}_t\}_{t=1}^T\) generated by r.v.s \(\{Y_{k}^s\}_{k \in \mathcal{K}, s \leq t}\) and \(\{R_{k}^s\}_{k \in \mathcal{K}, s \leq t}\). The corruption \(c_{k}^m\) becomes deterministic conditioned on \(\mathcal{F}_{t-1}\), and since \(\mathbb{E}\left[Y_{k}^t | \mathcal{F}_{t-1}\right] = p_{k}^m\), we have:
    \begin{align*}
        \mathbb{E}\left[X_{t} | \mathcal{F}_{t-1}\right] = \mathbb{E}\left[Y_{k}^t - p_{k}^m | \mathcal{F}_{t-1}\right]\cdot c_{k}^t = 0.
    \end{align*}

    As \(\left|X_{t}\right| \leq 1\), using a Freedman-type concentration inequality introduced in \citeauthor{beygelzimer2011contextual}, the predictive quadratic variation of this martingale can be bounded as:
    \begin{gather*}
        \Pr\left[\sum_{t\in E^m} X_{t} \geq V + \ln \frac{4}{\beta}\right] \leq \frac{\beta}{4},
    \end{gather*}
    where
    \begin{align*}
        V = & \sum_{t \in E^m}\mathbb{E}\left[X_t^2 | \mathcal{F}_{t-1}\right] \leq \sum_{t \in E^m} \left|c_{k}^t\right|\text{Var}\left(Y_{k}^t\right) \leq p_{k}^m\sum_{t \in E^m} \left|c_{k}^t\right|.
    \end{align*}
    Therefore, we obtain that with a probability of \(\frac{\beta}{4}\):
    \begin{align*}
        \frac{B_{k}^m}{p_{k}^mT^m} & \overset{(a)}\ge \frac{p_{k}^m}{p_{k}^mT^m}\sum_{t \in E^m} c_{k}^t + \frac{1}{p_{k}^mT^m} \left(V + \ln{\frac{4}{\beta}}\right) \\
                                   & \ge 2\frac{p_{k}^m}{p_{k}^mT^m}\sum_{t \in E^m} \left|c_{k}^t\right| + \frac{1}{p_{k}^mT^m} \ln{\frac{4}{\beta}},
    \end{align*}
    where (a) is because \(\sum_{t \in E^m}X_t = \sum_{t \in E^m}(Y_{k}^t - p_{k}^m)\cdot c_{k}^t = B_{k}^m - {p_{k}^m}\sum_{t \in E^m} c_{k}^t\).

    We also define the corruption in epoch \(m\)'s rewards as \(C^m = \sum_{t \in E^m}\max_{k \in \mathcal{K}} |c_{k}^t|\), therefore we can conclude that \(\sum_{t \in E^m} \left|c_{k}^t\right| \leq C^m\). We choose a parameter \(\beta \geq 4e^{(-\lambda/16)}\), therefore \(p_{k}^mT^m \geq \frac{2^{-2(m - 1)}}{2^6K}\lambda K 2^{2(m - 1)} \geq 16\ln{\left(4/\beta\right)}\). Then we can rewrite the same bound as:
    \begin{align}
        \label{eqn:B_corr_2_SA}
        \frac{B_{k}^m}{p_{k}^mT^m}\ge 2\frac{C^m}{T^m} + \sqrt{\frac{\ln{\frac{4}{\beta}}}{16p_{k}^mT^m}}.
    \end{align}
    \eqref{eqn:B_corr_2_SA} holds for \(-\frac{B_{k}^m}{p_{k}^mT^m}\) with the same probability, Therefore we have:
    \begin{align}
        \label{eqn:B_SA}
        Pr\left[\left|\frac{B_{k}^m}{p_{k}^mT^m}\right| \ge 2\frac{C^m}{T^m} + \sqrt{\frac{\ln{\frac{4}{\beta}}}{16p_{k}^mT^m}}\right] \le \frac{\beta}{2}.
    \end{align}

    \item
    \paragraph{Combining the two small probability bounds}Combining \eqref{eqn:A2_SA} and \eqref{eqn:B_SA}, we have:
    \begin{align*}
        Pr\left[\left|r_{k}^m - \mu_k\right| \geq \frac{2C^m}{T^m} + \sqrt{4\frac{\ln{\frac{4}{\beta}}}{p_{k}^mT^m}}\right] \le \beta.
    \end{align*}
    Then we set \(\beta = \delta/(2K\log{T})\), as this value satisfies \(\beta \geq 4e^{-\lambda/16}\), we have:
    \begin{align*}
        \sqrt{4\frac{\ln{\frac{4}{\beta}}}{p_{k}^mT^m}} = \sqrt{\frac{4\ln{(8k\log T/\delta)}}{p_k^m \times 2^{18}\ln{(8k\log T/\delta)}K2^{2(m - 1)}}} \le \frac{1}{16}\sqrt{\frac{2^6 K}{2^{-2(m - 1)} (\Delta_k^m)^{-2}K2^{2(m - 1)}}}
        \le \frac{\Delta_k^m}{16}
    \end{align*}
    \begin{align*}
        Pr\left[\left|r_{k}^m - \mu_k\right| \geq \frac{2C^m}{T^m} + \frac{\Delta_{k}^m}{16}\right] \leq \delta/(2K\log{T}).
    \end{align*}
    \item
    \begin{claim}
        \begin{align}
            \Pr\left[\Tilde{n}_{k}^m \geq 2 \cdot p_{k}^mT^m\right] \leq \beta
        \end{align}
    \end{claim}

    \begin{proof}
        Again, we can use a Chernoff-Hoeffding bound on the r.v. representing the actual number of pulls of arm \(k\) by agent \(\ell\) in eopch \(m\), which is: \(\tilde{n}_{k}^m \coloneqq \sum_{t \in E^m} Y_{k}^t\). The expected value of this r.v. is \(\mathbb{E}\left[\tilde{n}_{k}^m\right] = {p_{k}^mT^m}\). The probability that the r.v. is more than twice its expectation is at most: \(2\exp{\left(-\frac{p_{k}^mT^m}{3}\right)} \leq 2\exp{\left(-\frac{\lambda}{3}\right)} \leq 4\exp{\left(\frac{-\lambda}{16}\right)} \leq \beta\).
    \end{proof}

    Therefore using a union bound, we have:
    \begin{align}\label{eq:lem2_1_SA}
        \Pr\bigg[ & \forall k\in \mathcal{K}, m \in \{1, 2, \dots, M\}: \left|r_{k}^m - \mu_k\right| \geq \frac{2C^m}{T^m} + \frac{\Delta_{k}^m}{16} \text{ and } \Tilde{n}_{k}^m \geq 2 \cdot p_{k}^mT^m \bigg] \leq \delta.
    \end{align}

\end{proof}

% \textbf{Lemma 5.}
\begin{lemma}
    Suppose that \(\mathcal{E}\) happens, then for all epochs \(m\):
    \label{lem:5_SA}
    \begin{align}
        -\frac{2C^m}{T^m} - \frac{\Delta^{m - 1}_{k_{*}}}{8} \leq r_{*}^m - \mu_{*} \leq \frac{2C^m}{T^m}.
    \end{align}
\end{lemma}


\begin{proof}
    We know that \(r_{*}^m = \max_{k\in\mathcal{K}}{\{r_{k}^m - \frac{1}{16}\Delta_{k}^{m - 1}\}}\) and therefore \(r_{*}^m \geq r_{k_{*}}^m - \frac{1}{16}\Delta_{k_{*}}^{m - 1}\). Considering the lower bound implied by \(\mathcal{E}\) we have:
    \begin{align*}
        -\frac{2C^m}{T^m} - \frac{\Delta_{k_{*}}^{m - 1}}{8} \leq r_{*}^m - \mu_{*},
    \end{align*}
    We also know that:
    \begin{align*}
        r_{*}^m & = \max_{k\in\mathcal{K}}{\{r_{k}^m - \frac{1}{16}\Delta_{k}^{m - 1}\}}                                                      \\
                & \leq \max_{k\in\mathcal{K}}\{2\frac{C^m}{T^m} + \frac{1}{16}\Delta_{k}^{m - 1} + \mu_{k} - \frac{1}{16}\Delta_{k}^{m - 1}\} \\
                & \leq \mu_{*} + \frac{2C^m}{T^m}.
    \end{align*}
    Therefore the lemma is proved.
\end{proof}

Then we define \(\rho^m\) as:
\begin{equation}\label{eq:rho_SA}
    \rho^m = \sum_{s = 1}^{m}\frac{C^s}{8^{m - s}T^s}.
\end{equation}

\begin{lemma}
    \label{lem:6_SA}
    Suppose that \(\mathcal{E}\) happens, then for all epochs \(m\), arm \(k\), and agent \(\ell\):
    \begin{align}
        \Delta_{k}^m \leq 2(\Delta_{k} + 2^{-m} + \rho^m).
    \end{align}
\end{lemma}



\begin{proof}
    We prove this by induction on \(m\). For \(m = 1\), the claim is true for all \(k\), as \(\Delta_{k}^m \leq 1 \leq 2\cdot2^{-m}\).

    Suppose that the claim holds for \(m - 1\). Using Lemma~\ref{lem:5_SA} and the definition  of the event \(\mathcal{E}\), we write:
    \begin{equation}
        % \resizebox{.94\linewidth}{!}{
        \begin{split}
            \quad r_{*}^m - r_{k}^m & = (r_{*}^m - \mu_{*}) + (\mu_{*} - \mu_k) + (\mu_k - r_{k}^m)                                                                                          \\
                                    & \overset{(a)}\leq \frac{2C^m}{T^m} + \Delta_{k} + \frac{2C^m}{T^m} + \frac{\Delta^{m - 1}_{k}}{16}                                                     \\
                                    & \overset{(b)}\leq \Delta_{k} + \frac{4C^m}{T^m} + \frac{1}{8}\left(\Delta_{k} + 2^{-(m-1)} + \sum_{s = 1}^{m-1}\frac{C^{s}}{8^{(m - 1) - s}T^s}\right) \\
                                    & \leq 2\left(\Delta_{k} + 2^{-m} + \sum_{s = 1}^{m}\frac{C^{s}}{8^{m - s}T^s}\right),
        \end{split}
        % }
    \end{equation}
    where inequality (a) holds because \((r_{*}^m - \mu_{*})\) is bound using Lemma~\ref{lem:5_SA}, and \((\mu_k - r_{k}^m)\) is bound following the assumption of event \(\mathcal{E}\). Also, inequality (b) holds due to the induction's hypothesis.
    Therefore Lemma~\ref{lem:6_SA} is proved.
\end{proof}


\begin{lemma}
    \label{lem:7_SA}
    Suppose that \(\mathcal{E}\) happens, then for all epochs \(m\), arm \(k\), and agent \(\ell\):
    \begin{align}
        \Delta_{k}^m \geq \frac{1}{2} \Delta_{k} - 3\rho^m -\frac{3}{4}2^{-m}.
    \end{align}
\end{lemma}

\begin{proof}
    \begin{align*}
        \Delta_{k}^m  \geq r_{*}^m - r_{k}^m
         & \overset{(a)}\geq \left(\mu_{*} - \frac{2C^m}{T^m} - \frac{\Delta^{m - 1}_{k_{*}}}{8}\right) - \left(\mu_k + \frac{2C^m}{T^m} + \frac{\Delta^{m - 1}_{k}}{16}\right) \\
         & \overset{(b)}\geq \Delta_{k} - \frac{4C^m}{T^m} - \left(\frac{3}{8}\rho^{m-1} + \frac{3}{8}2^{-(m - 1)} + \frac{1}{8}\Delta_{k}\right)                               \\
         & \geq \frac{1}{2} \Delta_{k} - 3\sum_{s = 1}^{m}\frac{C^s}{8^{m - s}T^s} -\frac{3}{4}2^{-m}.
    \end{align*}
    where (a) holds because \(r_{*}^m\) can be bound using Lemma~\ref{lem:5_SA}, and \(r_{k}^m\) is bound due to event \(\mathcal{E}\), and (b) is because of Lemma~\ref{lem:6_SA}.
\end{proof}
\subsubsection{Proof for Theorem~\ref{theo:3}}
We decompose the total regret of each agent across epochs and within epochs, to the arms pulled. There are \(\tilde{n}^m_{k}\) pulls of arm \(k\) in epoch \(m\), each causing a regret of \((\mu_{*} - \mu_k)\). Thus the total regret can be written as:
\begin{align*}
    \sum_{m = 1}^{M}{\sum_{k \in \mathcal{K}}{(\mu_{*} - \mu_k)\tilde{n}^m_{k}}}
     & \overset{(a)}\leq 2\sum_{m = 1}^{M}{\sum_{k \in \mathcal{K}}{(\mu_{*} - \mu_k){p^m_{k}T^m}}}
    \\
     & = 2\sum_{m = 1}^{M}{\sum_{k \in \mathcal{K}}{\Delta_{k}{p^m_{k}T^m}}},
\end{align*}
where inequality (a) holds under event \(\mathcal{E}\) defined in~\eqref{eq:event-E_SA}.

Fix an epoch \(m\) and an arm \(k\) and denote \(\mathcal{R}^m_{k} := \Delta_{k}{p^m_{k}T^m}\) as the approximate regret for \((m, k)\). Consider the three following cases:

\paragraph{Case 1} \(0 \leq \Delta_{k} \leq 4/2^{m}\).
In this case we can upper bound \(p^m_{k}T^m \leq \frac{2^7}{A^m} \lambda K 2^{2(m - 1)}\), which follows:
\begin{align*}
    \mathcal{R}_{k}^m \leq \Delta_{k} \times \frac{2^7}{A^m} \lambda K2^{2(m - 1)} \leq 2^5 \frac{K}{A^m} \frac{16\lambda}{(\Delta_{k})^2} = 2^9 \frac{K}{A^m} \frac{\lambda}{\Delta_k}
\end{align*}

Therefore

\begin{align}
    \mathcal{R}_{\mathcal{A}}
     & \le \sum_{m = 1}^M2^9\frac{K}{A^m} \sum_{k \in \mathcal{A}^m} \frac{\lambda}{\Delta_k}
    \\
     & = O\left(\log(\frac{8K\log T}{\delta})\sum_{m = 1}^M\frac{K}{A^m}\sum_{k \in \mathcal{A}^m}\frac{1}{\Delta_k}\right)
    \\
     & = O\left(\log(\frac{8K\log T}{\delta})\log T\frac{K}{\Delta_{\min}}\right)
\end{align}


\paragraph{Case 2} \(\Delta_{k} > 4/2^{m}\) and \(\rho^m < \Delta_{k}/32\). In this case we can write:
\begin{align*}
    \Delta_{k}^{m-1} & \overset{(a)}\geq \frac{1}{2} \Delta_{k} - 3\rho^{m-1} -\frac{3}{4}2^{-(m-1)}                   \\
                     & \geq \Delta_{k} \left( \frac{1}{2} - \frac{3}{32} - \frac{3}{8} \right) = \frac{\Delta_{k}}{32}
    \ge \frac{1}{2^{m +3}},
\end{align*}
where inequality (a) holds for Lemma~\ref{lem:7_SA}. As \(\Delta_{k}^{m-1} \ge \frac{1}{2^{m +3}}\), we can infer that \(k \in \mathcal{B}^m\).

Therefore we can bound \(\mathcal{R}_{k}^m\) as:
\begin{align*}
    \mathcal{R}_{k}^m \leq \Delta_kp_k^mT^m \leq \Delta_k \frac{2^{-2(m - 1)}(\Delta_k^{m-1})^{-2}}{K}\lambda K 2^{2(m - 1)} \le \frac{2^{10}\lambda}{\Delta_{k}}
\end{align*}

Therefore

\begin{align}
    \mathcal{R}_{\mathcal{B}} & \le 2^{10}\sum_{m = 1}^M \sum_{k \in \mathcal{B}^m}\frac{\lambda}{\Delta_{k}}                                      \\
                              & = O\left(\log\left(\frac{8K\log T}{\delta}\right)\sum_{m=1}^M\sum_{k \in \mathcal{B}^m}\frac{1}{\Delta_{k}}\right) \\
                              & = O\left(\log\left(\frac{8K\log T}{\delta}\right) \log T \frac{K}{\Delta_{\min}}\right)
\end{align}
\paragraph{Case 3} \(\Delta_{k} > 4/2^{m}\) and \(\rho^m \geq \Delta_{k}/32\). Therefore \(\Delta_{k} \leq 32 \rho^m\). Hence, if \(k \in \mathcal{B}^m\), we have
\begin{align*}
    \mathcal{R}_{k}^m \leq \Delta_kp_k^mT^m \le 32\rho^m\frac{1}{K}\lambda K2^{2(m -1)}
    % {\lambda\Delta_{k}2^{2(m - 1)}} \leq {8\frac{\lambda}{L_k}\rho^{m-1}2^{2m}}.
\end{align*}

Therefore
\begin{align}
    \mathcal{R}_{\mathcal{B}} & \leq \sum_{m = 1}^M\sum_{k \in \mathcal{B}^m}8\lambda\rho^{m-1}2^{2m} = \sum_{m = 1}^M |\mathcal{B}^m| 8\lambda\rho^{m-1}2^{2m}\nonumber                                                                                                                           \\
                              & \overset{\eqref{eq:rho_d_2}}= \sum_{m = 1}^{M} 2^{2m}8\lambda|\mathcal{B}^m| \sum_{s = 1}^{m-1}\frac{2C^{s}}{8^{m - s - 1}T^s} = \sum_{s = 1}^{M - 1} 8\lambda\mathcal|{B}^s|C^s \sum_{m = s + 1}^{M} \frac{2^{2m}}{8^{m - 1 - s}\lambda K 2^{2(s - 1)}} \nonumber \\
                              & \overset{(a)}= \sum_{s = 1}^{M - 1} 16|\mathcal{B}^m|\frac{C^s}{K} \sum_{m = s+1}^{M} \frac{4^{m - 1 - s}}{8^{m - 1 - s}}\nonumber                                                                                                                                 \\
                              & \le \sum_{s = 1}^{M - 1} 16 \frac{|\mathcal{B}^m|}{K} \times C^s\label{eq:case3_B},
\end{align}
where (a) is because \(T^m = \lambda K 2^{2(m - 1)}\).

On the other hand if \(k \in \mathcal{A}^m\), we have
\begin{align*}
    \mathcal{R}_{k}^m \leq \Delta_kp_k^mT^m \le 32\rho^m\frac{1}{|\mathcal{A}^m|}\lambda K2^{2(m -1)}
    % {\lambda\Delta_{k}2^{2(m - 1)}} \leq {8\frac{\lambda}{L_k}\rho^{m-1}2^{2m}}.
\end{align*}

Therefore following the same analysis leading to \eqref{eq:case3_B}, we have
\begin{align}
    \mathcal{R}_{\mathcal{A}} & \leq \sum_{m = 1}^M\sum_{k \in \mathcal{A}^m}\frac{K}{|\mathcal{A}^m|}8\lambda\rho^{m-1}2^{2m} = \sum_{m = 1}^M 8\lambda\rho^{m-1}2^{2m} \sum_{k \in \mathcal{A}^m}\frac{K}{|\mathcal{A}^m|} = \sum_{m = 1}^M 8K\lambda\rho^{m-1}2^{2m} \nonumber \\
                              & \overset{\eqref{eq:rho_d_2}}= \sum_{m = 1}^{M} 8K\lambda 2^{2m} \sum_{s = 1}^{m-1}\frac{2C^{s}}{8^{m - s - 1}T^s} = \sum_{s = 1}^{M - 1} 16 K\frac{C^s}{T^s} \sum_{m = s + 1}^{M} \frac{2^{2m}}{8^{m - 1 - s} K 2^{2(s - 1)}} \nonumber           \\
                              & \overset{(a)}= \sum_{s = 1}^{M - 1} 16C^s \sum_{m = s+1}^{M} \frac{4^{m - 1 - s}}{8^{m - 1 - s}} \le \sum_{s = 1}^{M - 1} 16C^s\label{eq:case3_A},
\end{align}

Therefore the second part of the aggregated regret can be written as:
\begin{align}
    \sum_{m = 1}^{M} \sum_{k \in \mathcal{A}^m} 32\rho^m\frac{1}{|\mathcal{A}^m|}\lambda K2^{2(m -1)} + \sum_{m = 1}^{M}\sum_{k \in \mathcal{B}^m} 32\rho^m\lambda 2^{2(m -1)} \\
    \sum_{s = 1}^{M - 1} 16 \left(\frac{|\mathcal{B}^m|}{K} + 1\right) \times C^s \le 32 C = O(C).
\end{align}


Hence, the total aggregated regret can be bounded as follows, with probability at least \(1 - \delta\).
\begin{align}
    O\left(C + \log(\frac{8K\log T}{\delta})\log T\frac{K}{\Delta_{\min}}\right).
\end{align}
\newpage

\section{Multi-Agent (Homogeneous)}
We define an event \(\mathcal{E}\) such as:
\begin{align}\label{eq:event-E_MA}
    \mathcal{E} \coloneqq \left\{\forall \ell \in \mathcal{L}, \forall k\in \mathcal{K}_\ell, m \in \{1, \dots, M\} : \left|r_{k}^m - \mu_k\right| \le 2\frac{C^m}{L_kT^m} + \frac{\Delta_{k}^{m-1}}{16} \text{ and } \Tilde{n}_{k, \ell}^m \le {2 p^m_{k, \ell}T^m} \right\},
\end{align}
where \(C^m\) is the total corruption in epoch \(m\), and \(\Tilde{n}_{k, \ell}^m\) is the actual number of pulls of arm \(k\) in epoch \(m\) by agent \(\ell\).

% such that \(C = \sum_{\ell \in \mathcal{L}} \sum_{m = 1}^M C_\ell^m\)

\begin{lemma}\label{lem:4_MA}
    It holds that:
    \begin{align}
        \Pr[\mathcal{E}] \geq 1 - \delta.
    \end{align}
\end{lemma}


\begin{proof}
    % \(\beta \geq 4e^{-\frac{\lambda}{16L}}\), where \(L\) is the total number of agents.
    % For any fixed \(\ell \in \mathcal{L}\), \(k \in \mathcal{K}_{\ell}\), and \(m\) we have:
    \item
    \paragraph{Decomposing \(\pmb{r_{k}^m}\)}For this proof, we condition on all random variables before some fixed epoch \(m\) and agent \(\ell\), so that \(p^m_{k, \ell}\) is a deterministic quantity. At each step in this epoch, agent \(\ell\) picks arm \(k\) with probability \(p_{k}^m\). Let \(Y_{k, \ell}^t\) be an indicator for arm \(k\) being pulled in step \(t\) by agent \(\ell\). Let \(R_{k, \ell}^t\) be the stochastic reward of arm \(k\) on step \(t\) for agent \(\ell\). and \(c^t_{k, \ell} \coloneqq \tilde{R}_{k, \ell}^t - R_{k, \ell}^t\) be the corruption added to arm \(k\) by the adversary in step \(t\) for agent \(\ell\). Note that \(c^t_{k, \ell}\) may depend on all the stochastic rewards up to (and including) round \(t\), and also on all previous choices of the algorithm (though not the choice at step \(t\)). Finally, we denote \(E^m\) to be the \(T^m\) timesteps in epoch \(m\), then we define a random variable \(r_{k}^m\) as follows:
    \begin{equation}
        r_{k}^m = \frac{1}{Lp_{k}^mT^m}\sum_{\ell \in \mathcal{L}}\sum_{t \in E^m}Y_{k, \ell}^t\left(R_{k, \ell}^t + c_{k, \ell}^t\right).
    \end{equation}
    Let us break this sum into two:
    \begin{align*}
        A_{k}^m & = \sum_{\ell \in \mathcal{L}}\sum_{t \in E^m}Y_{k, \ell}^tR_{k, \ell}^t  \\
        B_{k}^m & = \sum_{\ell \in \mathcal{L}}\sum_{t \in E^m}Y_{k, \ell}^tc_{k, \ell}^t.
    \end{align*}

    \item
    \paragraph{Bounding the first and the second part} To \textbf{bound the first part}, we first note that:
    \begin{align*}
        \mathbb{E}\left[A_{k}^m\right] = LT^mp_{k}^m\mu_k,
    \end{align*}
    Therefore, according to the Chernoff-Hoeffding bound \cite{dubhashi2009concentration}, and because \(\mu_k \le 1\), for \(\beta \leq 1\) we have:
    \begin{align*}
        Pr\left[\left|\frac{A_{k}^m}{Lp_{k}^mT^m} - \mu_k\right| \geq \sqrt{\frac{3\ln{\frac{4}{\beta}}}{Lp_{k}^mT^m}}\right] \leq \frac{\beta}{2}.
    \end{align*}

    Next, we aim to \textbf{bound the second part}. To this end, we define the sequence of r.v.s, \(\{X_{t'}\}_{t'\in[1,\dots, LT]}\), where \(X_{t'} = \left(Y_{k, \ell}^t - p_{k}^m\right)\cdot c_{k, \ell}^t\) for all \(t'\), where \(t = \lceil  t'/L \rceil\), and \(\ell = t' \text{ mod } t\). Then \(\{X_{t'}\}_{t'\in[1,\dots, LT]}\) is a martingale sequence with respect to the filtration \(\{\mathcal{F}_t\}_{t=1}^T\) generated by r.v.s \(\{Y_{k, h}^s\}_{h \in L, k \in \mathcal{K}_h, s \leq t}\) and \(\{R_{k, h}^s\}_{h \in L, k \in \mathcal{K}_h, s \leq t}\). The corruption \(c_{k, \ell}^m\) becomes deterministic conditioned on \(\mathcal{F}_{t-1}\), and since \(\mathbb{E}\left[Y_{k, \ell}^t | \mathcal{F}_{t-1}\right] = p_{k}^m\), we have:
    \begin{align*}
        \mathbb{E}\left[X_{t'} | \mathcal{F}_{t-1}\right] = \sum_{\ell \in \mathcal{L}}\mathbb{E}\left[Y_{k, \ell}^t - p_{k}^m | \mathcal{F}_{t-1}\right]\cdot c_{k, \ell}^t = 0.
    \end{align*}

    As \(\left|X_{t'}\right| \leq 1\), using a Freedman-type concentration inequality introduced in \citeauthor{beygelzimer2011contextual}, the predictive quadratic variation of this martingale can be bounded as:
    \begin{gather*}
        \Pr\left[\sum_{t'} X_{t} \geq V + \ln \frac{4}{\beta}\right] \leq \frac{\beta}{4},
    \end{gather*}
    where
    \begin{align*}
        V = & \sum_{\ell \in \mathcal{L}}\sum_{t \in E^m}\mathbb{E}\left[X_{t'}^2 | \mathcal{F}_{t-1}\right] \leq \sum_{\ell \in \mathcal{L}}\sum_{t \in E^m} \left|c_{k, \ell}^t\right|\text{Var}\left(Y_{k, \ell}^t\right) \leq p_{k}^m\sum_{\ell \in \mathcal{L}}\sum_{t \in E^m} \left|c_{k, \ell}^t\right|.
    \end{align*}
    Therefore, we obtain that with a probability of \(\frac{\beta}{4}\):
    \begin{align*}
        \frac{B_{k}^m}{Lp_{k}^mT^m} & \overset{(a)}\ge \frac{p_{k}^m}{Lp_{k}^mT^m}\sum_{\ell \in \mathcal{L}}\sum_{t \in E^m} c_{k, \ell}^t + \frac{1}{Lp_{k}^mT^m} \left(V + \ln{\frac{4}{\beta}}\right) \\
                                    & \ge 2\frac{p_{k}^m}{Lp_{k}^mT^m}\sum_{\ell \in \mathcal{L}}\sum_{t \in E^m} \left|c_{k, \ell}^t\right| + \frac{1}{Lp_{k}^mT^m} \ln{\frac{4}{\beta}},
    \end{align*}
    where (a) is because \(\sum_{t'}X_{t'} = \sum_{t \in E^m}\sum_{\ell \in \mathcal{L}}(Y_{k, \ell}^t - p_{k}^m)\cdot c_{k, \ell}^t = B_{k}^m - {p_{k}^m}\sum_{t \in E^m}\sum_{\ell \in \mathcal{L}} c_{k, \ell}^t\).

    We also define the total corruption on epoch \(m\)'s rewards as \(C^m = \sum_{t \in E^m}\sum_{\ell \in \mathcal{L}}\max_{k \in \mathcal{K}} |c_{k, \ell}^t|\), therefore we can conclude that \(\sum_{t \in E^m} \sum_{\ell \in \mathcal{L}} \left|c_{k, \ell}^t\right| \leq C^m\). We choose a parameter \(\beta \geq 4e^{(-\lambda/16)}\), therefore \(p_{k}^mT^m \geq \frac{2^{-2(m - 1)}}{2^6K}\frac{\lambda K 2^{2(m - 1)}}{L} \geq \frac{16}{L}\ln{\left(4/\beta\right)}\). Then we can rewrite the same bound as:
    \begin{align}
        \label{eqn:B_corr_2_MA}
        \frac{B_{k}^m}{Lp_{k}^mT^m}\ge 2\frac{C^m}{LT^m} + \sqrt{\frac{\ln{\frac{4}{\beta}}}{16Lp_{k}^mT^m}}.
    \end{align}
    \eqref{eqn:B_corr_2_MA} holds for \(-\frac{B_{k}^m}{Lp_{k}^mT^m}\) with the same probability, Therefore we have:
    \begin{align*}
        Pr\left[\left|\frac{B_{k}^m}{Lp_{k}^mT^m}\right| \ge 2\frac{C^m}{LT^m} + \sqrt{\frac{\ln{\frac{4}{\beta}}}{16Lp_{k}^mT^m}}\right] \leq \frac{\beta}{2}.
    \end{align*}
    \item
    \paragraph{Combining the two small probability bounds}Combining \eqref{eqn:A2_MA} and \eqref{eqn:B_MA}, we have:
    \begin{align*}
        Pr\left[\left|r_{k}^m - \mu_k\right| \geq \frac{2C^m}{LT^m} + \sqrt{\frac{4\ln{\frac{4}{\beta}}}{Lp_{k}^mT^m}}\right] \leq \beta.
    \end{align*}
    Then we set \(\beta = \delta/(2K\log{T})\), as this value satisfies \(\beta \geq 4e^{-\lambda/16}\), we have:
    \begin{align*}
        \sqrt{4\frac{\ln{\frac{4}{\beta}}}{Lp_{k}^mT^m}} = \sqrt{\frac{4\ln{(8k\log T/\delta) \times L}}{Lp_{k}^m \times 2^{18}\ln{(8k\log T/\delta)}K2^{2(m - 1)}}} \le \sqrt{\frac{2^6 KL}{L2^{16}2^{-2(m - 1)} (\Delta_k^m)^{-2}K2^{2(m - 1)}}}
        \le \frac{\Delta_k^m}{16}
    \end{align*}
    \begin{align*}
        Pr\left[\left|r_{k}^m - \mu_k\right| \geq \frac{2C^m}{LT^m} + \frac{\Delta_{k}^m}{16}\right] \leq \delta/(2K\log{T}).
    \end{align*}
    \item
    \begin{claim}
        \begin{align}
            \Pr\left[\Tilde{n}_{k, \ell}^m \geq 2 \cdot p_{k}^mT^m\right] \leq \beta
        \end{align}
    \end{claim}

    \begin{proof}
        Again, we can use a Chernoff-Hoeffding bound on the r.v. representing the actual number of pulls of arm \(k\) by agent \(\ell\) in eopch \(m\), which is: \(\tilde{n}_{k, \ell}^m \coloneqq \sum_{t \in E^m} Y_{k, \ell}^t\). The expected value of this r.v. is \(\mathbb{E}\left[\tilde{n}_{k, \ell}^m\right] = {p_{k}^mT^m}\). The probability that the r.v. is more than twice its expectation is at most: \(2\exp{\left(-\frac{p_{k}^mT^m}{3}\right)} \leq 2\exp{\left(-\frac{\lambda}{3}\right)} \leq 4\exp{\left(\frac{-\lambda}{16}\right)} \leq \beta\).
    \end{proof}

    Therefore using a union bound, we have:
    \begin{align}\label{eq:lem2_1_MA}
        \Pr\bigg[ & \forall \ell\in \mathcal{L}, \forall k\in \mathcal{K}_\ell, m \in \{1, \dots, M\}: \left|r_{k}^m - \mu_k\right| \geq \frac{2C^m}{LT^m} + \frac{\Delta_{k}^m}{16} \text{ and } \Tilde{n}_{k, \ell}^m \geq 2 \cdot p_{k}^mT^m \bigg] \leq \delta.
    \end{align}

\end{proof}

% \textbf{Lemma 5.}
\begin{lemma}
    Suppose that \(\mathcal{E}\) happens, then for all epochs \(m\):
    \label{lem:5_MA}
    \begin{align}
        -\frac{2C^m}{LT^m} - \frac{\Delta^{m - 1}_{k_{*}}}{8} \leq r_{*}^m - \mu_{*} \leq \frac{2C^m}{LT^m}.
    \end{align}
\end{lemma}


\begin{proof}
    We know that \(r_{*}^m = \max_{k\in\mathcal{K}}{\{r_{k}^m - \frac{1}{16}\Delta_{k}^{m - 1}\}}\) and therefore \(r_{*}^m \geq r_{k_{*}}^m - \frac{1}{16}\Delta_{k_{*}}^{m - 1}\), where \(k_*\) is the arm with the largest global mean, \(\mu_*\). Considering the lower bound implied by \(\mathcal{E}\) we have:
    \begin{align*}
        -\frac{2C^m}{LT^m} - \frac{\Delta_{k_{*}}^{m - 1}}{8} \leq r_{*}^m - \mu_{*},
    \end{align*}
    We also know that:
    \begin{align*}
        r_{*}^m & = \max_{k\in\mathcal{K}}{\{r_{k}^m - \frac{1}{16}\Delta_{k}^{m - 1}\}}                                                       \\
                & \leq \max_{k\in\mathcal{K}}\{2\frac{C^m}{LT^m} + \frac{1}{16}\Delta_{k}^{m - 1} + \mu_{k} - \frac{1}{16}\Delta_{k}^{m - 1}\} \\
                & \leq \mu_{*} + \frac{2C^m}{LT^m}.
    \end{align*}
    Therefore the lemma is proved.
\end{proof}

Then we define \(\rho^m\) as:
\begin{equation}\label{eq:rho_MA}
    \rho^m = \sum_{s = 1}^{m}\frac{C^s}{8^{m - s}LT^s}.
\end{equation}

\begin{lemma}
    \label{lem:6_MA}
    Suppose that \(\mathcal{E}\) happens, then for all epochs \(m\) and arm \(k\):
    \begin{align}
        r_{*}^m - r_{k}^m \leq 2(\Delta_{k} + 2^{-m} + \rho^m).
    \end{align}
\end{lemma}



\begin{proof}
    We prove this by induction on \(m\). For \(m = 1\), the claim is true for all \(k\) and \(\ell\), as \(\Delta_{k}^m = 1 \le 2\cdot2^{-m}\).

    Suppose that the claim holds for \(m - 1\). Using Lemma~\ref{lem:5_MA} and the definition  of the event \(\mathcal{E}\), we write:
    \begin{equation}
        % \resizebox{.94\linewidth}{!}{
        \begin{split}
            \quad r_{*}^m - r_{k}^m & = (r_{*}^m - \mu_{*}) + (\mu_{*} - \mu_k) + (\mu_k - r_{k}^m)                                                                                            \\
                                    & \overset{(a)}\leq \frac{2C^m}{LT^m} + \Delta_{k} + \frac{2C^m}{LT^m} + \frac{\Delta^{m - 1}_{k}}{16}                                                     \\
                                    & \overset{(b)}\leq \Delta_{k} + \frac{4C^m}{LT^m} + \frac{1}{8}\left(\Delta_{k} + 2^{-(m-1)} + \sum_{s = 1}^{m-1}\frac{C^{s}}{8^{(m - 1) - s}LT^s}\right) \\
                                    & \leq 2\left(\Delta_{k} + 2^{-m} + \sum_{s = 1}^{m}\frac{C^{s}}{8^{m - s}LT^s}\right),
        \end{split}
        % }
    \end{equation}
    where inequality (a) holds because \((r_{*}^m - \mu_{*})\) is bound using Lemma~\ref{lem:5_MA}, and \((\mu_k - r_{k}^m)\) is bound following the assumption of event \(\mathcal{E}\). Also, inequality (b) holds due to the induction's hypothesis.
    Therefore Lemma~\ref{lem:6_MA} is proved.
\end{proof}


\begin{lemma}
    \label{lem:7_MA}
    Suppose that \(\mathcal{E}\) happens, then for all epochs \(m\) and arm \(k\):
    \begin{align}
        r_{*}^m - r_{k}^m \geq \frac{1}{2} \Delta_{k} - 3\rho^m -\frac{3}{4}2^{-m}.
    \end{align}
\end{lemma}

\begin{proof}
    \begin{align*}
        r_{*}^m - r_{k}^m
         & \overset{(a)}\geq \left(\mu_{*} - \frac{2C^m}{LT^m} - \frac{\Delta^{m - 1}_{k_{*}}}{8}\right) - \left(\mu_k + \frac{2C^m}{LT^m} + \frac{\Delta^{m - 1}_{k}}{16}\right) \\
         & \overset{(b)}\geq \Delta_{k} - \frac{4C^m}{LT^m} - \left(\frac{3}{8}\rho^{m-1} + \frac{3}{8}2^{-(m - 1)} + \frac{3}{8}\Delta_{k}\right)                                \\
         & \geq \frac{1}{2} \Delta_{k} - 3\sum_{s = 1}^{m}\frac{C^s}{8^{m - s}LT^s} -\frac{3}{4}2^{-m}.
    \end{align*}
    where (a) holds because \(r_{*}^m\) can be bound using Lemma~\ref{lem:5_MA}, and \(r_{k}^m\) is bound due to event \(\mathcal{E}\), and (b) is because of Lemma~\ref{lem:6_MA}.
\end{proof}

\subsubsection{Proof for Theorem~\ref{theo:3}}
We decompose the total regret of each agent across epochs and within epochs, to the arms pulled. There are \(\tilde{n}^m_{k, \ell}\) pulls of arm \(k\) in epoch \(m\) by agent \(\ell\), each causing a regret of \((\mu_{*} - \mu_k)\). Thus the total regret can be written as:
\begin{align*}
    \sum_{m = 1}^{M}{\sum_{\ell \in \mathcal{L}}\sum_{k \in \mathcal{K}_\ell}{(\mu_{*} - \mu_k)\tilde{n}^m_{k, \ell}}} & \overset{(a)}\leq 2\sum_{m = 1}^{M}\sum_{\ell \in \mathcal{L}}{\sum_{k \in \mathcal{K}_\ell}{(\mu_{*} - \mu_k){p^m_{k}T^m}}} \\
                                                                                                                       & = 2\sum_{m = 1}^{M}\sum_{\ell \in \mathcal{L}}{\sum_{k \in \mathcal{K}_\ell}{\Delta_{k}{p^m_{k}T^m}}},
\end{align*}
where inequality (a) holds under event \(\mathcal{E}\) defined in~\eqref{eq:event-E_MA}.

Fix an epoch \(m\), an agnet \(\ell\), and an arm \(k\) and denote \(\mathcal{R}^m_{k, \ell} := \Delta_{k}{p^m_{k}T^m}\) as the approximate regret for this \((m ,\ell, k)\) triad. Consider the three following cases:

\paragraph{Case 1} \(0 \leq \Delta_{k} \leq 4/2^{m}\).
In this case, if \(k \in \mathcal{A}^m\), we can write
\begin{align*}
    \mathcal{R}_{k, \ell}^m \leq \Delta_{k} \times \frac{2^7}{|\mathcal{A}^m|} \lambda \frac{K}{L}2^{2(m - 1)} \leq 2^5 \frac{K}{L|\mathcal{A}^m|} \frac{16\lambda}{(\Delta_{k})^2} = 2^9 \frac{K}{L|\mathcal{A}^m|} \frac{\lambda}{\Delta_k}
\end{align*}

Therefore

\begin{align}
    \mathcal{R}_{\mathcal{A}, 1} & \le \sum_{m = 1}^M \sum_{\ell \in \mathcal{L}} 2^9\frac{K}{L|\mathcal{A}^m|} \sum_{k \in \mathcal{A}^m} \frac{\lambda}{\Delta_k}                               \\
                                 & = O\left(\log(\frac{8K\log T}{\delta})\sum_{m = 1}^M \sum_{\ell \in \mathcal{L}} \frac{K}{L|\mathcal{A}^m|}\sum_{k \in \mathcal{A}^m}\frac{1}{\Delta_k}\right) \\
                                 & = O\left(\log(\frac{8K\log T}{\delta})\log T\frac{K}{\Delta_{\min}}\right).
\end{align}

And if \(k \in \mathcal{B}^m\), we have
\begin{align*}
    \mathcal{R}_{k, \ell}^m \leq \Delta_{k} \times \frac{2^6 \times 2^{-2(m - 1)}}{K} \lambda \frac{K}{L}2^{2(m - 1)} \leq 2^8\frac{\lambda}{L}2^{-m}
\end{align*}
Therefore
\begin{align}
    \mathcal{R}_{\mathcal{B}, 1} & \le \sum_{m = 1}^M \sum_{\ell \in \mathcal{L}} \sum_{k \in \mathcal{B}^m} 2^8\frac{\lambda}{L}2^{-m} \\
                                 & = O\left(K\log(\frac{8K\log T}{\delta})\log T\right).
\end{align}
\paragraph{Case 2} \(\Delta_{k} > 4/2^{m}\) and \(\rho^m < \Delta_{k}/32\). In this case we can write:
\begin{align*}
    \Delta_{k}^{m-1} \ge r_{*}^m - r_{k}^m & \overset{(a)}\geq \frac{1}{2} \Delta_{k} - 3\rho^{m-1} -\frac{3}{4}2^{-(m-1)}                                            \\
                                           & \geq \Delta_{k} \left( \frac{1}{2} - \frac{3}{32} - \frac{3}{8} \right) = \frac{\Delta_{k}}{32} \ge \frac{1}{2^{m + 3}},
\end{align*}
where inequality (a) holds for Lemma~\ref{lem:7_MA}. As \(r_{*}^m - r_{k}^m \ge \frac{1}{2^{m + 3}}\), \(k \in \mathcal{B}^m\) for all \(\ell \in \mathcal{L}_k\).

Therefore we can bound \(\mathcal{R}_{k}^m\) as:
\begin{align*}
    \mathcal{R}_{k}^m \leq \Delta_kp_k^mT^m \leq \Delta_k \frac{2^{-2(m - 1)}(\Delta_k^{m-1})^{-2}}{K}\lambda \frac{K}{L} 2^{2(m - 1)} \le \frac{2^{10}\lambda}{L\Delta_{k}}
\end{align*}

Therefore

\begin{align}
    \mathcal{R}_{\mathcal{B}, 2} & \le 2^{10}\sum_{m = 1}^M \sum_{\ell \in \mathcal{L}}\sum_{k \in \mathcal{B}^m}\frac{\lambda}{L\Delta_{k}}            \\
                                 & = O\left(\log\left(\frac{8K\log T}{\delta}\right)L\sum_{m=1}^M\sum_{k \in \mathcal{B}^m}\frac{1}{L\Delta_{k}}\right) \\
                                 & = O\left(\log\left(\frac{8K\log T}{\delta}\right) \log T \frac{K}{\Delta_{\min}}\right)
\end{align}
\paragraph{Case 3} \(\Delta_{k} > 4/2^{m}\) and \(\rho^m \geq \Delta_{k}/32\). Therefore \(\Delta_{k} \leq 32 \rho^m\). Hence, if \(k \in \mathcal{B}^m\), we have
\begin{align*}
    \mathcal{R}_{k}^m \leq \Delta_kp_k^mT^m \le 32\rho^m\frac{1}{K}\lambda \frac{K}{L}2^{2(m -1)}
    % {\lambda\Delta_{k}2^{2(m - 1)}} \leq {8\frac{\lambda}{L_k}\rho^{m-1}2^{2m}}.
\end{align*}

Therefore
\begin{align}
    \mathcal{R}_{\mathcal{B}, 3} & \leq \sum_{m = 1}^M\sum_{\ell \in \mathcal{L}}\sum_{k \in \mathcal{B}^m}8\lambda\rho^{m-1}2^{2m} = \sum_{m = 1}^M |\mathcal{B}^m| 8\lambda\rho^{m-1}2^{2m}\nonumber                                                                                                              \\
                                 & \overset{\eqref{eq:rho_d_2}}= \sum_{m = 1}^{M} 2^{2m}8\lambda|\mathcal{B}^m| \sum_{s = 1}^{m-1}\frac{2C^{s}}{8^{m - s - 1}LT^s} = \sum_{s = 1}^{M - 1} 8{\lambda}|\mathcal{B}^s|C^s \sum_{m = s + 1}^{M} \frac{2^{2m}}{8^{m - 1 - s}L\frac{\lambda}{L} K 2^{2(s - 1)}} \nonumber \\
                                 & \overset{(a)}= \sum_{s = 1}^{M - 1} 16|\mathcal{B}^m|\frac{C^s}{K} \sum_{m = s+1}^{M} \frac{4^{m - 1 - s}}{8^{m - 1 - s}}\nonumber                                                                                                                                               \\
                                 & \le \sum_{s = 1}^{M - 1} 16 \frac{|\mathcal{B}^m|}{K} \times C^s\label{eq:case3_B},
\end{align}
where (a) is because \(T^m = \lambda \frac{K}{L} 2^{2(m - 1)}\).

On the other hand if \(k \in \mathcal{A}^m\), we have
\begin{align*}
    \mathcal{R}_{k}^m \leq \Delta_kp_k^mT^m \le 32\rho^m\frac{1}{|\mathcal{A}^m|}\lambda \frac{K}{L}2^{2(m -1)}
    % {\lambda\Delta_{k}2^{2(m - 1)}} \leq {8\frac{\lambda}{L_k}\rho^{m-1}2^{2m}}.
\end{align*}

Therefore following the same analysis leading to \eqref{eq:case3_B}, we have
\begin{align}
    \mathcal{R}_{\mathcal{A}, 3} & \leq \sum_{m = 1}^M\sum_{\ell \in \mathcal{L}}\sum_{k \in \mathcal{A}^m}\frac{K}{|\mathcal{A}^m|}8{\lambda}\rho^{m-1}2^{2m} = \sum_{m = 1}^M 8{\lambda}\rho^{m-1}2^{2m} \sum_{k \in \mathcal{A}^m}\frac{K}{|\mathcal{A}^m|} = \sum_{m = 1}^M 8K{\lambda}\rho^{m-1}2^{2m} \nonumber \\
                                 & \overset{\eqref{eq:rho_d_2}}= \sum_{m = 1}^{M} 8K{\lambda} 2^{2m} \sum_{s = 1}^{m-1}\frac{2C^{s}}{8^{m - s - 1}T^s} = \sum_{s = 1}^{M - 1} 16 K{\lambda} C^s \sum_{m = s + 1}^{M} \frac{2^{2m}}{8^{m - 1 - s} KL\frac{\lambda}{L} 2^{2(s - 1)}} \nonumber                          \\
                                 & \overset{(a)}= \sum_{s = 1}^{M - 1} 16C^s \sum_{m = s+1}^{M} \frac{4^{m - 1 - s}}{8^{m - 1 - s}} \le \sum_{s = 1}^{M - 1} 16C^s\label{eq:case3_A},
\end{align}

Therefore the second part of the aggregated regret can be written as:
\begin{align}
    \sum_{m = 1}^{M} \sum_{k \in \mathcal{A}^m} 32\rho^m\frac{1}{|\mathcal{A}^m|}\lambda K2^{2(m -1)} + \sum_{m = 1}^{M}\sum_{k \in \mathcal{B}^m} 32\rho^m\lambda 2^{2(m -1)} \\
    \sum_{s = 1}^{M - 1} 16 \left(\frac{|\mathcal{B}^m|}{K} + 1\right) \times C^s \le 32 C = O(C).
\end{align}


Hence, the total aggregated regret can be bounded as follows, with probability at least \(1 - \delta\).
\begin{align}
    O\left(C + \log(\frac{8K\log T}{\delta})\log T\frac{K}{\Delta_{\min}}\right).
\end{align}
\newpage





















\section{Multi-Agent (Heterogeneous)}
We define an event \(\mathcal{E}\) such as:
\begin{align}\label{eq:event-E_MA}
    \mathcal{E} \coloneqq \left\{\forall \ell \in \mathcal{L}, \forall k\in \mathcal{K}_\ell, m \in \{1, \dots, M\} : \left|r_{k}^m - \mu_k\right| \le 2^{13}\frac{C^m}{L_{\min}T^m} + \frac{\Delta_{k}^{m-1}}{16} \text{ and } \Tilde{n}_{k, \ell}^m \le {2 p^m_{k, \ell}T^m} \right\},
\end{align}
where \(C^m\) is the total corruption in epoch \(m\), and \(\Tilde{n}_{k, \ell}^m\) is the actual number of pulls of arm \(k\) in epoch \(m\) by agent \(\ell\).

% such that \(C = \sum_{\ell \in \mathcal{L}} \sum_{m = 1}^M C_\ell^m\)

\begin{lemma}\label{lem:4_MA}
    It holds that:
    \begin{align}
        \Pr[\mathcal{E}] \geq 1 - \delta.
    \end{align}
\end{lemma}


\begin{proof}
    % \(\beta \geq 4e^{-\frac{\lambda}{16L}}\), where \(L\) is the total number of agents.
    % For any fixed \(\ell \in \mathcal{L}\), \(k \in \mathcal{K}_{\ell}\), and \(m\) we have:
    \item
    \paragraph{Decomposing \(\pmb{r_{k}^m}\) for \(\pmb{k \in A^m}\)}For this proof, we condition on all random variables before some fixed epoch \(m\) and agent \(\ell\), so that \(p^m_{k, \ell}\) is a deterministic quantity. At each step in this epoch, agent \(\ell\) picks arm \(k\) with probability \(p_{k, \ell}^m\). Let \(Y_{k, \ell}^t\) be an indicator for arm \(k\) being pulled in step \(t\) by agent \(\ell\). Let \(R_{k, \ell}^t\) be the stochastic reward of arm \(k\) on step \(t\) for agent \(\ell\). and \(c^t_{k, \ell} \coloneqq \tilde{R}_{k, \ell}^t - R_{k, \ell}^t\) be the corruption added to arm \(k\) by the adversary in step \(t\) for agent \(\ell\). Note that \(c^t_{k, \ell}\) may depend on all the stochastic rewards up to (and including) round \(t\), and also on all previous choices of the algorithm (though not the choice at step \(t\)). Finally, we denote \(E^m\) to be the \(T^m\) timesteps in epoch \(m\), then we define a random variable \(r_{k}^m\) as follows
    \begin{equation}
        r_{k}^m = \frac{\sum_{\ell \in \mathcal{L}_k}{|\mathcal{A}_\ell^m|}\sum_{t \in E^m}Y_{k, \ell}^t\left(R_{k, \ell}^t + c_{k, \ell}^t\right)}{\left(\sum_{\ell \in \mathcal{L}_k}{|\mathcal{A}_\ell^m|}p_{k, \ell}^m\right)T^m}.
    \end{equation}
    Let us break this sum into two and define
    \begin{align*}
        A_{k}^m & = {\sum_{\ell \in \mathcal{L}_k}\frac{|\mathcal{A}_\ell^m|}{|\mathcal{A}^m|}\sum_{t \in E^m}Y_{k, \ell}^t R_{k, \ell}^t}. \\
        B_{k}^m & = {\sum_{\ell \in \mathcal{L}_k}\frac{|\mathcal{A}_\ell^m|}{|\mathcal{A}^m|}\sum_{t \in E^m}Y_{k, \ell}^t c_{k, \ell}^t}.
    \end{align*}

    \item
    \paragraph{Bounding the first and the second part  for \(\pmb{k \in A^m}\)} To \textbf{bound the first part}, we first note that:
    \begin{align*}
        \mathbb{E}\left[A_{k}^m\right] = \left(\sum_{\ell \in \mathcal{L}_k}\frac{|\mathcal{A}_\ell^m|}{|\mathcal{A}^m|}p_{k, \ell}^m\right)T^m\mu_k,
    \end{align*}
    Therefore, according to the Chernoff-Hoeffding bound \cite{dubhashi2009concentration}, and because \(\mu_k \le 1\), for \(\beta \leq 1\) we have:
    \begin{align*}
        Pr\left[\left|\frac{A_{k}^m}{\left(\sum_{\ell \in \mathcal{L}_k}\frac{|\mathcal{A}_\ell^m|}{|\mathcal{A}^m|}p_{k, \ell}^m\right)T^m} - \mu_k\right| \geq \sqrt{\frac{3\ln{\frac{4}{\beta}}}{\left(\sum_{\ell \in \mathcal{L}_k}\frac{|\mathcal{A}_\ell^m|}{|\mathcal{A}^m|}p_{k, \ell}^m\right)T^m}}\right] \leq \frac{\beta}{2}.
    \end{align*}

    Next, we aim to \textbf{bound the second part}. To this end, we define the sequence of r.v.s, \(\{X_{t'}\}_{t'\in[1,\dots, LT]}\), where \(X_{t'} = \left(Y_{k, \ell}^t - p_{k, \ell}^m\right)\cdot \frac{|\mathcal{A}_\ell^m|}{|\mathcal{A}^m|}c_{k, \ell}^t\) for all \(t'\), where \(t = \lceil  t'/L \rceil\), and \(\ell = t' \text{ mod } t\). Then \(\{X_{t'}\}_{t'\in[1,\dots, LT]}\) is a martingale sequence with respect to the filtration \(\{\mathcal{F}_{t'}\}_{t'=1}^{LT}\) generated by r.v.s \(\{Y_{k, h}^s\}_{h \in L, k \in \mathcal{K}_h, s \leq t}\) and \(\{R_{k, h}^s\}_{h \in L, k \in \mathcal{K}_h, s \leq t}\). The corruption \(c_{k, \ell}^m\) becomes deterministic conditioned on \(\mathcal{F}_{t-1}\), and since \(\mathbb{E}\left[Y_{k, \ell}^t | \mathcal{F}_{t-1}\right] = p_{k, \ell}^m\), we have:
    \begin{align*}
        \mathbb{E}\left[X_{t'} | \mathcal{F}_{t-1}\right] = \sum_{\ell \in \mathcal{L}}\mathbb{E}\left[Y_{k, \ell}^t - p_{k, \ell}^m | \mathcal{F}_{t-1}\right]\cdot \frac{|\mathcal{A}_\ell^m|}{|\mathcal{A}^m|}c_{k, \ell}^t = 0.
    \end{align*}

    As \(\left|X_{t'}\right| \leq 1\), using a Freedman-type concentration inequality introduced in \citeauthor{beygelzimer2011contextual}, the predictive quadratic variation of this martingale can be bounded as:
    \begin{gather*}
        \Pr\left[\sum_{t'} X_{t} \geq V + \ln \frac{4}{\beta}\right] \leq \frac{\beta}{4},
    \end{gather*}
    where
    \begin{align*}
        V = & \sum_{\ell \in \mathcal{L}}\sum_{t \in E^m}\mathbb{E}\left[X_{t'}^2 | \mathcal{F}_{t-1}\right] \le \sum_{\ell \in \mathcal{L}}\sum_{t \in E^m} \frac{|\mathcal{A}_\ell^m|}{|\mathcal{A}^m|}\left|c_{k, \ell}^t\right|\text{Var}\left(Y_{k, \ell}^t\right) \leq \sum_{\ell \in \mathcal{L}} \frac{|\mathcal{A}_\ell^m|}{|\mathcal{A}^m|}p_{k, \ell}^m \sum_{t \in E^m} \left|c_{k, \ell}^t\right|.
    \end{align*}
    Therefore, we obtain that with a probability of \(\frac{\beta}{4}\):
    \begin{align*}
        \frac{B_{k}^m}{\left(\sum_{\ell \in \mathcal{L}_k}\frac{|\mathcal{A}_\ell^m|}{|\mathcal{A}^m|}p_{k, \ell}^m\right)T^m} & \overset{(a)}\ge \frac{\sum_{\ell \in \mathcal{L}} \frac{|\mathcal{A}_\ell^m|}{|\mathcal{A}^m|}p_{k, \ell}^m \sum_{t \in E^m} c_{k, \ell}^t}{\left(\sum_{\ell \in \mathcal{L}_k}\frac{|\mathcal{A}_\ell^m|}{|\mathcal{A}^m|}p_{k, \ell}^m\right)T^m} + \frac{1}{\left(\sum_{\ell \in \mathcal{L}_k}\frac{|\mathcal{A}_\ell^m|}{|\mathcal{A}^m|}p_{k, \ell}^m\right)T^m} \left(V + \ln{\frac{4}{\beta}}\right) \\
                                                                                                                               & \ge 2\frac{\sum_{\ell \in \mathcal{L}} {|\mathcal{A}_\ell^m|}p_{k, \ell}^m \sum_{t \in E^m} \left|c_{k, \ell}^t\right|}{\left(\sum_{\ell \in \mathcal{L}_k}{|\mathcal{A}_\ell^m|}p_{k, \ell}^m\right)T^m} + \frac{1}{\left(\sum_{\ell \in \mathcal{L}_k}\frac{|\mathcal{A}_\ell^m|}{|\mathcal{A}^m|}p_{k, \ell}^m\right)T^m} \ln{\frac{4}{\beta}},
    \end{align*}

    where (a) is because \(\sum_{t'}X_{t'} = \sum_{\ell \in \mathcal{L}}\sum_{t \in E^m}(Y_{k, \ell}^t - p_{k, \ell}^m)\cdot \frac{|\mathcal{A}_\ell^m|}{|\mathcal{A}^m|} c_{k, \ell}^t = B_{k}^m - \sum_{\ell \in \mathcal{L}} \frac{|\mathcal{A}_\ell^m|}{|\mathcal{A}^m|} p_{k, \ell}^m \sum_{t \in E^m} c_{k, \ell}^t\).

    We also define the total corruption on agent \(\ell\)'s rewards in epoch \(m\) as \(C^m_\ell = \sum_{t \in E^m}\max_{k \in \mathcal{K}} |c_{k, \ell}^t|\), therefore we can conclude that \(\sum_{\ell \in \mathcal{L}} \left|c_{k, \ell}^t\right| \leq C_\ell^m\). We choose a parameter \(\beta \geq 4e^{(-\lambda/16)}\), therefore
    \begin{align*}
        (\sum_{\ell \in \mathcal{L}_k}\frac{|\mathcal{A}_\ell^m|}{|\mathcal{A}^m|}p_{k, \ell}^m)T^m & \ge \sum_{\ell \in \mathcal{L}_k}(\frac{|\mathcal{A}_\ell^m|}{|\mathcal{A}^m|}\frac{(1 - 2^{-2}))}{|\mathcal{A}_\ell^m|})\frac{\lambda K 2^{2(m - 1)}}{L_{\min}} \\
                                                                                                    & \ge \frac{3L_{\min}}{4|\mathcal{A}^m|}\frac{2^{18}\ln(\frac{4}{\beta}) K 2^{2(m - 1)}}{L_{\min}}                                                                 \\
                                                                                                    & \ge 16\ln{\left(4/\beta\right)}.
    \end{align*}
    Then we can rewrite the same bound as:

    \begin{align}
        \label{eqn:B_corr_2_MA}
        \frac{B_{k}^m}{(\sum_{\ell \in \mathcal{L}_k}\frac{|\mathcal{A}_\ell^m|}{|\mathcal{A}^m|}p_{k}^m)T^m}\ge 2\frac{\sum_{\ell \in \mathcal{L}_k}p_{k, \ell}^m{|\mathcal{A}_\ell^m|}C^m_\ell}{(\sum_{\ell \in \mathcal{L}_k}p_{k}^m{|\mathcal{A}_\ell^m|})T^m} + \sqrt{\frac{\ln{\frac{4}{\beta}}}{16(\sum_{\ell \in \mathcal{L}_k}\frac{|\mathcal{A}_\ell^m|}{|\mathcal{A}^m|}p_{k}^m)T^m}}.
    \end{align}
    Furthermore, we can write
    \begin{align*}
        \frac{\sum_{\ell \in \mathcal{L}_k}{|\mathcal{A}_\ell^m|}p_{k, \ell}^mC^m_\ell}{(\sum_{\ell \in \mathcal{L}_k}{|\mathcal{A}_\ell^m|}p_{k}^m)T^m} \le \frac{\sum_{\ell \in \mathcal{L}_k}\frac{1}{|\mathcal{A}_\ell^m|}{|\mathcal{A}_\ell^m|}C^m_\ell}{(\sum_{\ell \in \mathcal{L}_k}{|\mathcal{A}_\ell^m|}\frac{3}{4|\mathcal{A}_\ell^m|})T^m} \le \frac{4}{3}\frac{C_\ell^m}{L_{\min}T^m}
    \end{align*}

    \eqref{eqn:B_corr_2_MA} holds for \(-\frac{B_{k}^m}{(\sum_{\ell \in \mathcal{L}_k}\frac{|\mathcal{A}_\ell^m|}{|\mathcal{A}^m|}p_{k}^m)T^m}\) with the same probability, Therefore we have:
    \begin{align*}
        Pr\left[\left|\frac{B_{k}^m}{(\sum_{\ell \in \mathcal{L}_k}\frac{|\mathcal{A}_\ell^m|}{|\mathcal{A}^m|}p_{k}^m)T^m}\right| \ge \frac{8}{3}\frac{C^m_\ell}{L_{\min}T^m} + \sqrt{\frac{\ln{\frac{4}{\beta}}}{16(\sum_{\ell \in \mathcal{L}_k}\frac{|\mathcal{A}_\ell^m|}{|\mathcal{A}^m|}p_{k}^m)T^m}}\right] \leq \frac{\beta}{2}.
    \end{align*}
    \item
    \paragraph{Combining the two small probability bounds  for \(\pmb{k \in A^m}\)} Combining \eqref{eqn:A2_MA} and \eqref{eqn:B_MA}, we have:
    \begin{align*}
        Pr\left[\left|r_{k}^m - \mu_k\right| \geq \frac{8}{3}\frac{C^m}{L_{\min}T^m} + \sqrt{\frac{4\ln{\frac{4}{\beta}}}{(\sum_{\ell \in \mathcal{L}_k}\frac{|\mathcal{A}_\ell^m|}{|\mathcal{A}^m|}p_{k}^m)T^m}}\right] \leq \beta.
    \end{align*}
    Then we set \(\beta = \delta/(2K\log{T})\), as this value satisfies \(\beta \geq 4e^{-\lambda/16}\), we have:
    \begin{align*}
        \sqrt{\frac{4\ln{\frac{4}{\beta}}}{(\sum_{\ell \in \mathcal{L}_k}\frac{|\mathcal{A}_\ell^m|}{|\mathcal{A}^m|}p_{k}^m)T^m}} & \le \sqrt{\frac{4\ln{(8k\log T/\delta)}\times L_{\min}}{(\sum_{\ell \in \mathcal{L}_k}\frac{3}{4|\mathcal{A}^m_\ell|}\frac{|\mathcal{A}^m_\ell|}{|\mathcal{A}^m|}) \times 2^{18}\ln{(8k\log T/\delta)}K2^{2(m - 1)}}} \\
                                                                                                                                   & = \sqrt{\frac{|\mathcal{A}^m|}{2^{14}K2^{2(m - 1)}}} \leq \frac{1}{16}\sqrt{\frac{1}{2^6}} \overset{(a)}{=} \frac{1}{16}\sqrt{(\Delta_k^m)^2},
    \end{align*}
    where (a) is due to the face that \(k \in \mathcal{A}^m\), therefore \(r_{*, max}^{m - 1} - r_k^{m - 1} \le 2^{-(m + 3)}\) and hence, \(\Delta_k^m = 2^{-3}\).
    Therefore we have:
    \begin{align*}
        Pr\left[\left|r_{k}^m - \mu_k\right| \geq \frac{8}{3}\frac{C^m}{L_{\min}T^m} + \frac{\Delta_{k}^m}{16}\right] \leq \delta/(2K\log{T}).
    \end{align*}
    \item

    \item
    \paragraph{Decomposing \(\pmb{r_{k}^m}\) for \(\pmb{k \in \mathcal{B}^m}\)}For this proof, we condition on all random variables before some fixed epoch \(m\) and agent \(\ell\), so that \(p^m_{k, \ell}\) is a deterministic quantity. At each step in this epoch, agent \(\ell\) picks arm \(k\) with probability \(p_{k, \ell}^m\). Let \(Y_{k, \ell}^t\) be an indicator for arm \(k\) being pulled in step \(t\) by agent \(\ell\). Let \(R_{k, \ell}^t\) be the stochastic reward of arm \(k\) on step \(t\) for agent \(\ell\). and \(c^t_{k, \ell} \coloneqq \tilde{R}_{k, \ell}^t - R_{k, \ell}^t\) be the corruption added to arm \(k\) by the adversary in step \(t\) for agent \(\ell\). Note that \(c^t_{k, \ell}\) may depend on all the stochastic rewards up to (and including) round \(t\), and also on all previous choices of the algorithm (though not the choice at step \(t\)). Finally, we denote \(E^m\) to be the \(T^m\) timesteps in epoch \(m\), then we define a random variable \(r_{k}^m\) as follows:
    \begin{equation}
        r_{k}^m = \frac{\sum_{\ell \in \mathcal{L}_k}{K_\ell}\sum_{t \in E^m}Y_{k, \ell}^t\left(R_{k, \ell}^t + c_{k, \ell}^t\right)}{\left(\sum_{\ell \in \mathcal{L}_k}{K_\ell}p_{k, \ell}^m\right)T^m}.
    \end{equation}
    Let us break this sum into two:


    \begin{align*}
        A_{k}^m & = {\sum_{\ell \in \mathcal{L}_k}\frac{K_\ell}{K}\sum_{t \in E^m}Y_{k, \ell}^t R_{k, \ell}^t}. \\
        B_{k}^m & = {\sum_{\ell \in \mathcal{L}_k}\frac{K_\ell}{K}\sum_{t \in E^m}Y_{k, \ell}^t c_{k, \ell}^t}.
    \end{align*}

    \item
    \paragraph{Bounding the first and the second part  for \(\pmb{k \in \mathcal{B}^m}\)} To \textbf{bound the first part}, we first note that:
    \begin{align*}
        \mathbb{E}\left[A_{k}^m\right] = \left(\sum_{\ell \in \mathcal{L}_k}\frac{K_\ell}{K}p_{k, \ell}^m\right)T^m\mu_k,
    \end{align*}
    Therefore, according to the Chernoff-Hoeffding bound \cite{dubhashi2009concentration}, and because \(\mu_k \le 1\), for \(\beta \leq 1\) we have:
    \begin{align*}
        Pr\left[\left|\frac{A_{k}^m}{\left(\sum_{\ell \in \mathcal{L}_k}\frac{K_\ell}{K}p_{k, \ell}^m\right)T^m} - \mu_k\right| \geq \sqrt{\frac{3\ln{\frac{4}{\beta}}}{\left(\sum_{\ell \in \mathcal{L}_k}\frac{K_\ell}{K}p_{k, \ell}^m\right)T^m}}\right] \leq \frac{\beta}{2}.
    \end{align*}

    Next, we aim to \textbf{bound the second part}. To this end, we define the sequence of r.v.s, \(\{X_{t'}\}_{t'\in[1,\dots, LT]}\), where \(X_{t'} = \left(Y_{k, \ell}^t - p_{k, \ell}^m\right)\cdot \frac{K_\ell}{K}c_{k, \ell}^t\) for all \(t'\), where \(t = \lceil  t'/L \rceil\), and \(\ell = t' \text{ mod } t\). Then \(\{X_{t'}\}_{t'\in[1,\dots, LT]}\) is a martingale sequence with respect to the filtration \(\{\mathcal{F}_{t'}\}_{t=1}^{LT}\) generated by r.v.s \(\{Y_{k, h}^s\}_{h \in L, k \in \mathcal{K}_h, s \leq t}\) and \(\{R_{k, h}^s\}_{h \in L, k \in \mathcal{K}_h, s \leq t}\). The corruption \(c_{k, \ell}^m\) becomes deterministic conditioned on \(\mathcal{F}_{t-1}\), and since \(\mathbb{E}\left[Y_{k, \ell}^t | \mathcal{F}_{t-1}\right] = p_{k, \ell}^m\), we have:
    \begin{align*}
        \mathbb{E}\left[X_{t'} | \mathcal{F}_{t-1}\right] = \sum_{\ell \in \mathcal{L}}\mathbb{E}\left[Y_{k, \ell}^t - p_{k, \ell}^m | \mathcal{F}_{t-1}\right]\cdot \frac{K_\ell}{K}c_{k, \ell}^t = 0.
    \end{align*}

    As \(\left|X_{t'}\right| \leq 1\), using a Freedman-type concentration inequality introduced in \citeauthor{beygelzimer2011contextual}, the predictive quadratic variation of this martingale can be bounded as:
    \begin{gather*}
        \Pr\left[\sum_{t'} X_{t} \geq V + \ln \frac{4}{\beta}\right] \leq \frac{\beta}{4},
    \end{gather*}
    where
    \begin{align*}
        V = & \sum_{\ell \in \mathcal{L}}\sum_{t \in E^m}\mathbb{E}\left[X_{t'}^2 | \mathcal{F}_{t-1}\right] \le \sum_{\ell \in \mathcal{L}}\sum_{t \in E^m} \frac{K_\ell}{K}\left|c_{k, \ell}^t\right|\text{Var}\left(Y_{k, \ell}^t\right) \leq \sum_{\ell \in \mathcal{L}}\frac{K_\ell}{K}p_{k, \ell}^m  \sum_{t \in E^m} \left|c_{k, \ell}^t\right|.
    \end{align*}
    Therefore, we obtain that with a probability of \(\frac{\beta}{4}\):
    \begin{align*}
        \frac{B_{k}^m}{\left(\sum_{\ell \in \mathcal{L}_k}\frac{K_\ell}{K}p_{k, \ell}^m\right)T^m} & \overset{(a)}\ge \frac{\sum_{\ell \in \mathcal{L}}\frac{K_\ell}{K}p_{k, \ell}^m  \sum_{t \in E^m} c_{k, \ell}^t}{\left(\sum_{\ell \in \mathcal{L}_k}\frac{K_\ell}{K}p_{k, \ell}^m\right)T^m} + \frac{1}{\left(\sum_{\ell \in \mathcal{L}_k}\frac{K_\ell}{K}p_{k, \ell}^m\right)T^m} \left(V + \ln{\frac{4}{\beta}}\right) \\
                                                                                                   & \ge 2\frac{\sum_{\ell \in \mathcal{L}}p_{k, \ell}^m {K_\ell} \sum_{t \in E^m} \left|c_{k, \ell}^t\right|}{\left(\sum_{\ell \in \mathcal{L}_k}{K_\ell}p_{k, \ell}^m\right)T^m} + \frac{1}{\left(\sum_{\ell \in \mathcal{L}_k}\frac{K_\ell}{K}p_{k, \ell}^m\right)T^m} \ln{\frac{4}{\beta}},
    \end{align*}

    where (a) is because \(\sum_{t'}X_{t'} = \sum_{\ell \in \mathcal{L}}\sum_{t \in E^m}(Y_{k, \ell}^t - p_{k, \ell}^m)\cdot \frac{K_\ell}{K} c_{k, \ell}^t = B_{k}^m - \sum_{\ell \in \mathcal{L}} \frac{K_\ell}{K}{p_{k, \ell}^m} \sum_{t \in E^m} c_{k, \ell}^t\).

    We also define the total corruption on agent \(\ell\)'s rewards in epoch \(m\) as \(C^m_\ell = \sum_{t \in E^m}\max_{k \in \mathcal{K}} |c_{k, \ell}^t|\), therefore we can conclude that \(\sum_{\ell \in \mathcal{L}} \left|c_{k, \ell}^t\right| \leq C_\ell^m\). We choose a parameter \(\beta \geq 4e^{(-\lambda/16)}\), therefore
    \begin{align*}
        (\sum_{\ell \in \mathcal{L}_k}\frac{K_\ell}{K}p_{k}^m)T^m & \ge \sum_{\ell \in \mathcal{L}_k}(\frac{K_\ell}{K}\frac{2^{-2m}}{2^6K_\ell}\frac{L_{\min}}{L_{k}})\frac{\lambda K 2^{2(m - 1)}}{L_{\min}} \\
                                                                  & = \frac{2^{-2m}L_{\min}}{2^6K}\frac{2^{18}\ln(\frac{4}{\beta}) K 2^{2(m - 1)}}{L_{\min}}                                                  \\
                                                                  & \ge 16\ln{\left(4/\beta\right)}.
    \end{align*}
    Then we can rewrite the same bound as:

    \begin{align}
        \label{eqn:B_corr_2_MA}
        \frac{B_{k}^m}{(\sum_{\ell \in \mathcal{L}_k}\frac{K_\ell}{K}p_{k}^m)T^m}\ge 2\frac{\sum_{\ell \in \mathcal{L}_k}{K_\ell}p_{k, \ell}^mC^m_\ell}{(\sum_{\ell \in \mathcal{L}_k}{K_\ell}p_{k}^m)T^m} + \sqrt{\frac{\ln{\frac{4}{\beta}}}{16(\sum_{\ell \in \mathcal{L}_k}{K_\ell}p_{k}^m)T^m}}.
    \end{align}
    Furthermore, we can write
    \begin{align*}
        \frac{\sum_{\ell \in \mathcal{L}_k}{K_\ell}p_{k, \ell}^mC^m_\ell}{(\sum_{\ell \in \mathcal{L}_k}{K_\ell}p_{k}^m)T^m} \le \frac{\sum_{\ell \in \mathcal{L}_k}\frac{2^{-2m}2^6}{K_\ell}{K_\ell}C^m_\ell}{(\sum_{\ell \in \mathcal{L}_k}{K_\ell}\frac{2^{-2m}}{2^6K_\ell})T^m} = 2^{12}\frac{C^m}{L_{\min}T^m}
    \end{align*}

    \eqref{eqn:B_corr_2_MA} holds for \(-\frac{B_{k}^m}{(\sum_{\ell \in \mathcal{L}_k}{K_\ell}p_{k}^m)T^m}\) with the same probability, Therefore we have:
    \begin{align*}
        Pr\left[\left|\frac{B_{k}^m}{(\sum_{\ell \in \mathcal{L}_k}\frac{K_\ell}{K}p_{k}^m)T^m}\right| \ge 2^{13}\frac{C^m_\ell}{L_{\min}T^m} + \sqrt{\frac{\ln{\frac{4}{\beta}}}{16(\sum_{\ell \in \mathcal{L}_k}\frac{K_\ell}{K}p_{k}^m)T^m}}\right] \leq \frac{\beta}{2}.
    \end{align*}
    \item
    \paragraph{Combining the two small probability bounds  for \(\pmb{k \in \mathcal{B}^m}\)} Combining \eqref{eqn:A2_MA} and \eqref{eqn:B_MA}, we have:
    \begin{align*}
        Pr\left[\left|r_{k}^m - \mu_k\right| \geq 2^{13}\frac{C^m}{L_{\min}T^m} + \sqrt{\frac{4\ln{\frac{4}{\beta}}}{(\sum_{\ell \in \mathcal{L}_k}\frac{K_\ell}{K}p_{k}^m)T^m}}\right] \leq \beta.
    \end{align*}
    Then we set \(\beta = \delta/(2K\log{T})\), as this value satisfies \(\beta \geq 4e^{-\lambda/16}\), we have:
    \begin{align*}
        \sqrt{\frac{4\ln{\frac{4}{\beta}}}{(\sum_{\ell \in \mathcal{L}_k}\frac{K_\ell}{K}p_{k}^m)T^m}} & = \sqrt{\frac{4\ln{(8k\log T/\delta)}\times L_{\min}}{(\sum_{\ell \in \mathcal{L}_k}\frac{L_{\min}}{L_k}\frac{2^{-2m}(\Delta_k^m)^{-2}}{2^6K_\ell}\frac{K_\ell}{K}) \times 2^{18}\ln{(8k\log T/\delta)}K2^{2(m - 1)}}} \\
                                                                                                       & = \sqrt{\frac{4L_{\min} \times K2^6(\Delta_k^m)^2}{L_{\min}2^{-2m} \times 2^{18}K2^{2(m - 1)}}} = \frac{\Delta_k^m}{16}.
    \end{align*}
    Therefore we have:
    \begin{align*}
        Pr\left[\left|r_{k}^m - \mu_k\right| \geq 2^{13}\frac{C^m}{L_{\min}T^m} + \frac{\Delta_{k}^m}{16}\right] \leq \delta/(2K\log{T}).
    \end{align*}
    \item


    \begin{claim}
        \begin{align}
            \Pr\left[\Tilde{n}_{k, \ell}^m \geq 2 \cdot p_{k, \ell}^mT^m\right] \leq \beta
        \end{align}
    \end{claim}

    \begin{proof}
        Again, we can use a Chernoff-Hoeffding bound on the r.v. representing the actual number of pulls of arm \(k\) by agent \(\ell\) in eopch \(m\), which is: \(\tilde{n}_{k, \ell}^m \coloneqq \sum_{t \in E^m} Y_{k, \ell}^t\). The expected value of this r.v. is \(\mathbb{E}\left[\tilde{n}_{k, \ell}^m\right] = {p_{k, \ell}^mT^m}\). The probability that the r.v. is more than twice its expectation is at most: \(2\exp{\left(-\frac{p_{k, \ell}^mT^m}{3}\right)} \leq 2\exp{\left(-\frac{\lambda}{3}\right)} \leq 4\exp{\left(\frac{-\lambda}{16}\right)} \leq \beta\).
    \end{proof}

    Therefore using a union bound, we have:
    \begin{align}\label{eq:lem2_1_MA}
        \Pr\bigg[ & \forall \ell\in \mathcal{L}, \forall k\in \mathcal{K}_\ell, m \in \{1, \dots, M\}: \left|r_{k}^m - \mu_k\right| \geq 2^{13}\frac{C^m}{L_{\min}T^m} + \frac{\Delta_{k}^m}{16} \text{ and } \Tilde{n}_{k, \ell}^m \geq 2 \cdot p_{k, \ell}^mT^m \bigg] \leq \delta.
    \end{align}

\end{proof}

% \textbf{Lemma 5.}
\begin{lemma}
    Suppose that \(\mathcal{E}\) happens, then for all epochs \(m\):
    \label{lem:5_MA}
    \begin{align}
        -2^{13}\frac{C^m}{L_{\min}T^m} - \frac{\Delta^{m - 1}_{k_{*}}}{8} \leq r_{*, \max}^m - \mu_{*} \leq 2^{13}\frac{C^m}{L_{\min}T^m}.
    \end{align}
\end{lemma}


\begin{proof}
    We know that \(r_{*, max}^m = \max_{k\in\mathcal{K}}{\{r_{k}^m - \frac{1}{16}\Delta_{k}^{m - 1}\}}\) and therefore \(r_{*, \max}^m \geq r_{k_{*}}^m - \frac{1}{16}\Delta_{k_{*}}^{m - 1}\), where \(k_*\) is the arm with the largest global mean, \(\mu_*\). Considering the lower bound implied by \(\mathcal{E}\) we have:
    \begin{align*}
        -2^{13}\frac{C^m}{L_{\min}T^m} - \frac{\Delta_{k_{*}}^{m - 1}}{8} \leq r_{*, \max}^m - \mu_{*},
    \end{align*}
    We also know that:
    \begin{align*}
        r_{*, \max}^m & = \max_{k\in\mathcal{K}}{\{r_{k}^m - \frac{1}{16}\Delta_{k}^{m - 1}\}}                                                                   \\
                      & \leq \max_{k\in\mathcal{K}}\{2^{13}\frac{C^m}{L_{\min}T^m} + \frac{1}{16}\Delta_{k}^{m - 1} + \mu_{k} - \frac{1}{16}\Delta_{k}^{m - 1}\} \\
                      & \leq \mu_{*} + 2^{13}\frac{C^m}{L_{\min}T^m}.
    \end{align*}
    Therefore the lemma is proved.
\end{proof}

Then we define \(\rho^m\) as:
\begin{equation}\label{eq:rho_MA}
    \rho^m = \sum_{s = 1}^{m}\frac{2C^s}{8^{m - s -4}L_{\min}T^s}.
\end{equation}

\begin{lemma}
    \label{lem:6_MA}
    Suppose that \(\mathcal{E}\) happens, then for all epochs \(m\) and arm \(k\):
    \begin{align}
        \Delta_{k}^m \leq 2(\Delta_{k} + \sqrt{\frac{L_{\min}}{L_{\max}}}2^{-m} + \rho^m + 2^{-4}).
    \end{align}
\end{lemma}



\begin{proof}
    We prove this by induction on \(m\). For \(m = 1\), the claim is true for all \(k\) and \(\ell\), as \(\Delta_{k}^m = 1 \le 2\cdot2^{-m}\).

    Suppose that the claim holds for \(m - 1\). Using Lemma~\ref{lem:5_MA} and the definition  of the event \(\mathcal{E}\), we write:
    \begin{equation}
        % \resizebox{.94\linewidth}{!}{
        \begin{split}
            \quad r_{*, \max}^m - r_{k}^m & = (r_{*, \max}^m - \mu_{*}) + (\mu_{*} - \mu_k) + (\mu_k - r_{k}^m)                                                                                                                                                       \\
                                          & \overset{(a)}\leq 2^{13}\frac{C^m}{L_{\min}T^m} + \Delta_{k} + 2^{13}\frac{C^m}{L_{\min}T^m} + \frac{\Delta^{m - 1}_{k}}{16}                                                                                              \\
                                          & \overset{(b)}\leq \Delta_{k} + \frac{2^{14}C^m}{L_{\min}T^m} + \frac{1}{8}\left(\Delta_{k} + \sqrt{\frac{L_{\min}}{L_{\max}}}2^{-(m-1)} + \sum_{s = 1}^{m-1}\frac{2C^{s}}{8^{(m - 1) - s - 4}L_{\min}T^s} + 2^{-4}\right) \\
                                          & \leq 2\left(\Delta_{k} + \sqrt{\frac{L_{\min}}{L_{\max}}}2^{-m} + \sum_{s = 1}^{m}\frac{2C^{s}}{8^{m - s -4}L_{\min}T^s} + 2^{-8}\right),
        \end{split}
        % }
    \end{equation}
    where inequality (a) holds because \((r_{*, \max}^m - \mu_{*})\) is bound using Lemma~\ref{lem:5_MA}, and \((\mu_k - r_{k}^m)\) is bound following the assumption of event \(\mathcal{E}\). Also, inequality (b) holds due to the induction's hypothesis. Finally, we know that \(\Delta_{k}^m \le \max\{2^{-3}, r_{*, \max}^m - r_{k}^m + 3 \cdot 2^{-7}\}\). Therefore
    \begin{align*}
        \Delta_{k}^m \le 2\left(\Delta_{k} + \sqrt{\frac{L_{\min}}{L_{\max}}}2^{-m} + \rho^m + 2^{-8}\right) + 3 \cdot 2^{-7} \le 2(\Delta_{k} + \sqrt{\frac{L_{\min}}{L_{\max}}}2^{-m} + \rho^m + 2^{-4})
    \end{align*}
    Therefore Lemma~\ref{lem:6_MA} is proved.
\end{proof}


\begin{lemma}
    \label{lem:7_MA}
    Suppose that \(\mathcal{E}\) happens, then for all epochs \(m\) and arm \(k\):
    \begin{align}
        \Delta_{k}^m \geq \frac{1}{2} \Delta_{k} - 3\rho^m -\frac{3}{4}\sqrt{\frac{L_{\min}}{L_{\max}}}2^{-m}.
    \end{align}
\end{lemma}

\begin{proof}
    \begin{align*}
        r_{*, \max}^m - r_{k}^m
         & \overset{(a)}\geq \left(\mu_{*} - 2^{13}\frac{C^m}{L_{\min}T^m} - \frac{\Delta^{m - 1}_{k_{*}}}{8}\right) - \left(\mu_k + 2^{13}\frac{C^m}{L_{\min}T^m} + \frac{\Delta^{m - 1}_{k}}{16}\right)      \\
         & \overset{(b)}\geq \Delta_{k} - \frac{2^{14}C^m}{L_{\min}T^m} - \left(\frac{3}{8}\rho^{m-1} + \frac{3}{8}\sqrt{\frac{L_{\min}}{L_{\max}}}2^{-(m - 1)} + \frac{3}{8}\Delta_{k} + 3\times2^{-7}\right) \\
         & \geq \frac{1}{2} \Delta_{k} - 3\sum_{s = 1}^{m}\frac{2C^s}{8^{m - s -4}L_{\min}T^s} -\frac{3}{4}\sqrt{\frac{L_{\min}}{L_{\max}}}2^{-m} -3\times2^{-7}.
    \end{align*}
    where (a) holds because \(r_{*, \max}^m\) can be bound using Lemma~\ref{lem:5_MA}, and \(r_{k}^m\) is bound due to event \(\mathcal{E}\), and (b) is because of Lemma~\ref{lem:6_MA}.
\end{proof}

\subsubsection{Proof for Theorem~\ref{theo:3}}
We decompose the total regret of each agent across epochs and within epochs, to the arms pulled. There are \(\tilde{n}^m_{k, \ell}\) pulls of arm \(k\) in epoch \(m\) by agent \(\ell\), each causing a regret of \((\mu_{*} - \mu_k)\). Thus the total regret can be written as:
\begin{align*}
    \sum_{m = 1}^{M}{\sum_{k \in \mathcal{K}}\sum_{\ell \in \mathcal{L}_k}{(\mu_{*, \ell} - \mu_k)\tilde{n}^m_{k, \ell}}} & \overset{(a)}\leq 2\sum_{m = 1}^{M}{\sum_{k \in \mathcal{K}}\sum_{\ell \in \mathcal{L}_k}{(\mu_{*, \ell} - \mu_k){p^m_{k, \ell}T^m}}}                                                                                           \\
                                                                                                                          & = 2\sum_{m = 1}^{M}{\sum_{k \in \mathcal{K}}\sum_{\ell \in \mathcal{L}_k}{\Delta_{k}{p^m_{k, \ell}T^m}}} - 2\sum_{m = 1}^{M}{\sum_{k \in \mathcal{K}}\sum_{\ell \in \mathcal{L}_k}{(\mu_* - \mu_{*, \ell}){p^m_{k, \ell}T^m}}},
\end{align*}
where inequality (a) holds under event \(\mathcal{E}\) defined in~\eqref{eq:event-E_MA}.

Fix an epoch \(m\), an agnet \(\ell\), and an arm \(k\) and denote \(\mathcal{R}^m_{k, \ell} := \Delta_{k}{p^m_{k, \ell}T^m}\) as the approximate regret for this \((m ,\ell, k)\) triad. Consider the three following cases:

\paragraph{Case 1} \(0 \leq \Delta_{k} \leq \frac{4}{2^{m}}\sqrt{\frac{L_{\min}}{L_k}}\).
In this case, if \(k \in \mathcal{A}^m\), we can write
\begin{align*}
    \mathcal{R}_{k, \ell}^m \leq \Delta_{k} \times \frac{1}{|\mathcal{A}^m|} \lambda \frac{K}{L_{\min}}2^{2(m - 1)} \leq 2^5 \Delta_k\frac{K}{L_{\min}|\mathcal{A}^m|} \frac{16\lambda}{(\Delta_{k})^2}\frac{L_{\min}}{L_{k}} = 2^9 \frac{K}{L_{k}|\mathcal{A}^m|} \frac{\lambda}{\Delta_k}
\end{align*}

Therefore

\begin{align}
    \mathcal{R}_{\mathcal{A}, 1} & \le \sum_{m = 1}^M 2^9\frac{K}{L_{k}|\mathcal{A}^m|} \sum_{k \in \mathcal{A}^m}\sum_{\ell \in \mathcal{L}_k} \frac{\lambda}{\Delta_k} \\
                                 & = O\left(\log(\frac{8K\log T}{\delta})\sum_{m = 1}^M
    \frac{K}{|\mathcal{A}^m|}\sum_{k \in \mathcal{A}^m}\frac{1}{\Delta_k}\right)                                                                                         \\
                                 & = O\left(\log(\frac{8K\log T}{\delta})\log T\frac{K}{\Delta_{\min}}\right).
\end{align}

And if \(k \in \mathcal{B}^m\), we have
\begin{align*}
    \mathcal{R}_{k, \ell}^m \leq \Delta_{k} \times \frac{2^6 \times 2^{-2m}}{K}{\frac{L_{\min}}{L_{k}}} \lambda \frac{K}{L_{\min}}2^{2(m - 1)} \leq 2^4\frac{\lambda}{L_{k}}2^{-m}
\end{align*}
Therefore
\begin{align}
    \mathcal{R}_{\mathcal{B}, 1} & \le \sum_{m = 1}^M \sum_{k \in \mathcal{B}^m} \sum_{\ell \in \mathcal{L}_k}2^4\frac{\lambda}{L_{k}}2^{-m} \\
                                 & = O\left(K\log(\frac{8K\log T}{\delta})\log T\right).
\end{align}


\paragraph{Case 2} \(\Delta_{k} > \frac{4}{2^{m}}\sqrt{\frac{L_{\min}}{L_k}}\) and \(\rho^{m - 1} < \Delta_{k}/32\). In this case we can write:
\begin{align*}
    r_{*, \max}^m - r_{k}^m & \overset{(a)}\geq \frac{1}{2} \Delta_{k} - 3\rho^{m-1} -\frac{3}{4}\sqrt{\frac{L_{\min}}{L_{\max}}}2^{-(m-1)} -3 \times 2^{-7}                     \\
                            & \geq \Delta_{k} \left( \frac{1}{2} - \frac{3}{32} - \frac{3}{8}\sqrt{\frac{L_{\min}}{L_{\max}}}\sqrt{\frac{L_k}{L_{\min}}}\right) -3 \times 2^{-7} \\
                            & \ge   \frac{\Delta_{k}}{32}-3 \times 2^{-7} \ge \frac{1}{2^{m + 3}}\sqrt{\frac{L_{\min}}{L_k}}-3 \times 2^{-7},
\end{align*}
where inequality (a) holds for Lemma~\ref{lem:7_MA}. As \(r_{*, \max}^m - r_{k}^m \ge \frac{1}{2^{m + 3}}\sqrt{\frac{L_{\min}}{L_{\max}}}-3 \times 2^{-7}\), \(k \in \mathcal{B}^m_\ell\) for all \(\ell \in \mathcal{L}_k\).
We also have \(\Delta_{k}^m = \max\{2^{-3}, r_{*, \max}^m - r_{k}^m + 3 \cdot 2^{-7}\} \ge r_{*, \max}^m - r_{k}^m + 3 \cdot 2^{-7} \ge \frac{\Delta_{k}}{32}-3 \cdot 2^{-7}+ 3 \cdot 2^{-7}\)
% \begin{align*}
%     \Delta_k^{m-1} \ge \sqrt{\frac{L_k}{L_{\min}}}\left(r_{*, \max}^m - r_{k}^m\right) \ge \frac{\Delta_{k}}{32}\sqrt{\frac{L_k}{L_{\min}}} 
% \end{align*}
Therefore we can bound \(\mathcal{R}_{k}^m\) as:
\begin{align*}
    \mathcal{R}_{k}^m \leq \Delta_kp_k^mT^m \leq \Delta_k \frac{2^{-2m}(\Delta_k^{m-1})^{-2}}{K}\frac{L_{\min}}{L_k}\lambda \frac{K}{L_{\min}} 2^{2(m - 1)} \le \frac{2^{6}\lambda}{\Delta_{k}L_k}
\end{align*}

Therefore

\begin{align}
    \mathcal{R}_{\mathcal{B}, 2} & \le 2^{10}\sum_{m = 1}^M \sum_{k \in \mathcal{B}^m}\sum_{\ell \in \mathcal{L}_k}\frac{\lambda}{L_k\Delta_{k}}           \\
                                 & = O\left(\log\left(\frac{8K\log T}{\delta}\right)\sum_{m=1}^M\sum_{k \in \mathcal{B}^m_\ell}\frac{1}{\Delta_{k}}\right) \\
                                 & = O\left(\log\left(\frac{8K\log T}{\delta}\right) \log T \frac{K}{\Delta_{\min}}\right)
\end{align}
\paragraph{Case 3} \(\Delta_{k} > \frac{4}{2^m}\sqrt{\frac{L_{\min}}{L_k}}\) and \(\rho^{m - 1} \geq \Delta_{k}/32\). Therefore \(\Delta_{k} \leq 32 \rho^{m - 1}\). Hence, if \(k \in \mathcal{B}^m\), we have
\begin{align*}
    \mathcal{R}_{k}^m \leq \Delta_kp_k^mT^m \le 32\rho^{m - 1}\frac{1}{K}\frac{L_{\min}}{L_k}\lambda \frac{K}{L_{min}}2^{2(m -1)}
    % {\lambda\Delta_{k}2^{2(m - 1)}} \leq {8\frac{\lambda}{L_k}\rho^{m-1}2^{2m}}.
\end{align*}

Therefore
\begin{align}
    \mathcal{R}_{\mathcal{B}, 3} & \leq \sum_{m = 1}^M\sum_{k \in \mathcal{B}^m}\sum_{\ell \in \mathcal{L}_k}8\frac{\lambda}{L_k}\rho^{m-1}2^{2m} = \sum_{m = 1}^M |\mathcal{B}^m| 8\lambda\rho^{m-1}2^{2m}\nonumber \\
                                 & \overset{\eqref{eq:rho_d_2}}= \sum_{m = 1}^{M} 2^{2m}8\lambda|\mathcal{B}^m| \sum_{s = 1}^{m-1}\frac{2C^{s}}{8^{m - s - 5}L_{\min}T^s}                                            \\
                                 & = \sum_{s = 1}^{M - 1} 8\lambda|\mathcal{B}^s|C^s \sum_{m = s + 1}^{M} \frac{2^{2m}L_{\min}}{8^{m - 5 - s}L_{\min}\lambda K 2^{2(s - 1)}} \nonumber                               \\
                                 & \overset{(a)}= \sum_{s = 1}^{M - 1} 16|\mathcal{B}^s|\frac{C^s}{K} \sum_{m = s+1}^{M} \frac{4^{m - 1 - s}}{8^{m - 5 - s}}\nonumber                                                \\
                                 & \le \sum_{s = 1}^{M - 1} 2^{16} \frac{|\mathcal{B}^s|}{K} \times C^s\label{eq:case3_B},
\end{align}
where (a) is because \(T^m = \lambda \frac{K}{L_{\min}} 2^{2(m - 1)}\).

On the other hand if \(k \in \mathcal{A}^m\), we have
\begin{align*}
    \mathcal{R}_{k}^m \leq \Delta_kp_k^mT^m \le 32\rho^{m - 1}\frac{1}{|\mathcal{A}^m|}\lambda \frac{K}{L_{\min}}2^{2(m -1)}
    % {\lambda\Delta_{k}2^{2(m - 1)}} \leq {8\frac{\lambda}{L_k}\rho^{m-1}2^{2m}}.
\end{align*}

Therefore following the same analysis leading to \eqref{eq:case3_B}, we have
\begin{align}
    \mathcal{R}_{\mathcal{A}} & \leq \frac{1}{L_{\min}}\sum_{m = 1}^M\sum_{k \in \mathcal{A}^m}\sum_{\ell \in \mathcal{L}_k}\frac{K}{|\mathcal{A}^m|}8\lambda\rho^{m-1}2^{2m}  = \frac{L_{\max}}{L_{\min}}\sum_{m = 1}^M 8\lambda\rho^{m-1}2^{2m} \sum_{k \in \mathcal{A}^m}\frac{K}{|\mathcal{A}^m|} = \frac{L_{\max}}{L_{\min}}\sum_{m = 1}^M 8K\lambda\rho^{m-1}2^{2m} \nonumber \\
                              & \overset{\eqref{eq:rho_d_2}}= \frac{L_{\max}}{L_{\min}}\sum_{m = 1}^{M} 8K\lambda 2^{2m} \sum_{s = 1}^{m-1}\frac{2C^{s}}{8^{m - s - 1}L_{\min}T^s} = \frac{L_{\max}}{L_{\min}}\sum_{s = 1}^{M - 1} 16 K\frac{C^s}{T^s} \sum_{m = s + 1}^{M} \frac{2^{2m}}{8^{m - 5 - s} L_{\min}K 2^{2(s - 1)}} \nonumber                                           \\
                              & \overset{(a)}= \frac{L_{\max}}{L_{\min}}\sum_{s = 1}^{M - 1} 16C^s \sum_{m = s+1}^{M} \frac{4^{m - 5 - s}}{8^{m - 5 - s}} \le \frac{L_{\max}}{L_{\min}}\sum_{s = 1}^{M - 1} 2^{16}C^s\label{eq:case3_A},
\end{align}


Hence, the total aggregated regret can be bounded as follows, with probability at least \(1 - \delta\).
\begin{align}
    R_{\mathcal{A}, 1} + R_{\mathcal{B}, 1} + R_{\mathcal{B}, 2} + R_{\mathcal{A}, 3} + R_{\mathcal{B}, 3} \le O\left(\frac{L_{\max}}{L_{\min}}C + \log(\frac{8K\log T}{\delta})\log T\frac{K}{\Delta_{\min}}\right).
\end{align}
\newpage







\color{blue}

\section{\lfbarbar}

\subsection{\lfbarbar regret upper bound}\label{appendix:a_1}

\subsubsection{Lemmas for Proving Theorem~\ref{theo:1}}

\begin{lemma}
    We can bound variable \(N_{\max}^m\) as:
    \begin{align}
        \frac{\lambda2^{2(m-1)}}{\hat L} \leq N_{\max}^{m} \leq K\lambda2^{2(m-1)},
    \end{align}
    where \(\hat L = \min_{\ell \in \mathcal{L}}\max_{k \in \mathcal{K}_{\ell}}{L_{k}}\). Also, the number of epochs \(M\) is:
    \[
        M = O\left(\log(\frac{T}{\lambda})\right),
    \]
    which is at most \(O(\log(T)\).
\end{lemma}


\begin{proof}
    For each agent \(\ell\), there exists an arm \(k_{\ell}^m\) achieving the reward \(r^m_{*, \ell}\) and fulfilling \(r^m_{*, \ell} - r^m_{k_{\ell}^m} \leq 0\). Therefore \(\Delta^m_{k_{\ell}^m, \ell} = 2^{-m}\). So we have:
    \begin{align*}
        N_\ell^{m + 1} \geq n^{m + 1}_{k_{\ell}^m, \ell} = \frac{\lambda\left(\Delta^m_{k_{\ell}^m, \ell}\right)^{-2}}{L_{k_{\ell}^m}} = \frac{\lambda2^{2m}}{L_{k_{\ell}^m}}.
    \end{align*}
    On the other hand, since that \(\Delta_{k, \ell}^{m} \geq 2^{-m}\), so for each \(k\) we have \(n^m_{k, \ell} \leq \frac{\lambda2^{2m}}{L_{k}}\). Hence, the lemma is proved. The bound on \(M\) follows the lower bound on \(N_{\max}^{m}\).

\end{proof}

We define an event \(\mathcal{E}\) such as:
\begin{align}\label{eq:event-E_d_2}
    \mathcal{E} \coloneqq \left\{\forall k\in \mathcal{K}, \ell\in \mathcal{L}_k, m \in \{1, 2, \dots, M\} : \left|r_{k}^m - \mu_k\right| \geq 2\max_{\ell \in \mathcal{L}}\frac{C^m_\ell}{N^m_{\max}} + \frac{\Delta_{k, \max}^{m-1}}{16} \text{ and } \Tilde{n}_{k, \ell}^m \geq {2 n_{k, \ell}^m} \right\},
\end{align}
where \(C_{\ell}^m\) is the total corruption on agent \(\ell\) in set in epoch \(m\), and \(\Tilde{n}_{k, \ell}^m\) is the actual number of pulls of arm \(k\) by agent \(\ell\) in epoch \(m\).

\begin{lemma}\label{lem:2_4}
    It holds that:
    \begin{align}
        \Pr[\mathcal{E}] \geq 1 - \delta.
    \end{align}
\end{lemma}


\begin{proof}
    % \(\beta \geq 4e^{-\frac{\lambda}{16L}}\), where \(L\) is the total number of agents.
    % For any fixed \(\ell \in \mathcal{L}\), \(k \in \mathcal{K}_{\ell}\), and \(m\) we have:
    \item
    \paragraph{Decomposing \(\pmb{r_{k}^m}\)}For this proof, we condition on all random variables before some fixed epoch \(m\), so that \(n^m_{k, \ell}\) , \(N_{\max}^m\) and \(T^{m-1}\) are deterministic quantities. At each step in this epoch, agent \(\ell\) picks arm \(k\) with probability \(q_{k, \ell}^m \coloneqq \frac{n^m_{k, \ell}}{N_{\max}^m}\). Let \(Y_{k, \ell}^m\) be an indicator for arm \(k\) being selected for agent \(\ell\) for epoch \(m\). Let \(R_{k, \ell}^t\) be the stochastic reward of arm \(k\) on step \(t\) for agent \(\ell\). and \(c^t_{k, \ell} \coloneqq \tilde{R}_{k, \ell}^t - R_{k, \ell}^t\) be the corruption added to arm \(k\) by the adversary in step \(t\) for agent \(\ell\). Note that \(c^t_{k, \ell}\) may depend on all the stochastic rewards up to (and including) round \(t\), and also on all previous choices of the algorithm (though not the choice at step \(t\). Finally, if we denote \(E^m = \{T^{m-1} + 1, . . . , T^{m}\}\) to be the \(N_{\max}^{m}\) timesteps in epoch \(m\), then we define a random variable \(r_{k}^m\) as follows:
    \begin{equation}
        r_{k}^m = \frac{1}{n_{k}^m}\sum_{\ell \in \mathcal{L}_k}\sum_{t \in E^m}Y_{k, \ell}^m(R_{k, \ell}^t + c_{k, \ell}^t).
    \end{equation}
    Let us break this sum into two:
    \begin{align*}
        A_{k}^m & = \sum_{\ell \in \mathcal{L}_k}\sum_{t \in E^m}Y_{k, \ell}^mR_{k, \ell}^t  \\
        B_{k}^m & = \sum_{\ell \in \mathcal{L}_k}\sum_{t \in E^m}Y_{k, \ell}^mc_{k, \ell}^t.
    \end{align*}


    \item
    \paragraph{Bounding the first and the second part} To \textbf{bound the first part}, we first note that:
    \begin{align*}
        \mathbb{E}\left[A_{k}^m\right] = \sum_{\ell \in \mathcal{L}_k}N^m_{\max}.\left(q_{k, \ell}^m\mu_k\right) = n_{k}^m\mu_k,
    \end{align*}
    Where \(n_{k}^m = \sum_{\ell \in \mathcal{L}_k}{n_{k, \ell}^m}\).
    Therefore, as the selection of arms for every agent is independent, according to the Hoeffding bound, for any \(\beta \leq 1\) we have:
    \begin{gather}
        \label{eqn:A_1}
        \Pr\left[\left|\frac{A_{k}^m}{n_{k}^m} - \mu_k\right| \geq \sqrt{\frac{3\ln{\frac{4}{\beta}}}{n_{k}^m}}\right]
        \leq 2\exp\left(\frac{6\mu_k\ln{\frac{\beta}{4}}}{n_k^m L_k (N_{\max}^m)^2}\right)
        \leq 2\exp\left(\frac{6\mu_{\min}\ln{\frac{\beta}{4}}}{LT^3}\right)
        \overset{(a)}\leq \frac{\beta}{2},
    \end{gather}
    where inequality (a) is because \(T \geq \sqrt[3]{\frac{6\mu_{\min}}{L}}\).

    Next, we aim to \textbf{bound the second part}. To this end, we define the sequence of r.v.s, \(\{X_t\}_{t = 1}^{T}\), where \(X_t = \sum_{\ell \in \mathcal{L}_k}(Y_{k, \ell}^m - q_{k, \ell}^m)\cdot c_{k, \ell}^t\). Then \(\{X_t\}_{t = 1}^{T}\) is a martingale difference sequence with respect to the filtration \(\{\mathcal{F}_t\}_{t = 1}^{T}\) generated by r.v.s \(\{Y_{k, h}^n\}_{h \in \mathcal{L}, k \in \mathcal{K}_h, s \leq m}\) and \(\{R_{k, h}^s\}_{h \in \mathcal{L}, k \in \mathcal{K}_h, s \leq t}\). The corruption \(c_{k, \ell}^t\) becomes deterministic conditioned on \(\mathcal{F}_{t-1}\), and since \(\mathbb{E}\left[Y_{k, \ell}^m | \mathcal{F}_{t-1}\right] = q_{k, \ell}^m\), we have:
    \begin{align*}
        \mathbb{E}\left[X_t | \mathcal{F}_{t-1}\right] = \sum_{\ell \in \mathcal{L}_k}\mathbb{E}\left[Y_{k, \ell}^m - q_{k, \ell}^m | \mathcal{F}_{t-1}\right]\cdot c_{k, \ell}^t = 0.
    \end{align*}
    Using a Freedman-type concentration inequality, the predictive quadratic variation of this martingale can be bounded as:
    \begin{gather*}
        \Pr\left[X_t \geq V + \ln \frac{4}{\beta}\right] \leq \frac{\beta}{4},
    \end{gather*}
    where
    \begin{align*}
        V = & \sum_{t \in E^m_\ell}\mathbb{E}\left[X_t^2 | \mathcal{F}_{t-1}\right] \leq \sum_{\ell\in \mathcal{L}_k}\text{Var}\left(Y_{k, \ell}^m\right)\sum_{t \in E^m_\ell} \left|c_{k, \ell}^t\right|\ \leq \sum_{\ell\in \mathcal{L}_k}q_{k, \ell}^m\sum_{t \in E^m_\ell} \left|c_{k, \ell}^t\right|.
    \end{align*}
    Therefore, we obtain that with a probability of \(1 - \frac{\beta}{4}\):
    \begin{align*}
        \frac{B_k^m}{n_{k}^m} & \overset{(a)}\leq \sum_{\ell\in \mathcal{L}_k}\frac{q_{k, \ell}^m}{n_{k}^m}\sum_{t \in E^m_\ell} c_{k, \ell}^t + \frac{1}{n_{k}^m} \left(V + \ln{\frac{4}{\beta}}\right) \\
                              & \leq 2\sum_{\ell\in \mathcal{L}_k}\frac{q_{k, \ell}^m}{n_{k}^m}\sum_{t \in E^m_\ell} \left|c_{k, \ell}^t\right| + \frac{1}{n_{k}^m} \ln{\frac{4}{\beta}},
    \end{align*}
    where (a) is because \(\sum_{\ell \in \mathcal{L}_k}\sum_{t \in E^m}X_t = \sum_{\ell \in \mathcal{L}_k}\sum_{t \in E^m}(Y_{k, \ell}^m - q_{k, \ell}^m)\cdot c_{k, \ell}^t = B_{k}^m - \sum_{\ell \in \mathcal{L}_k}{q_{k, \ell}^m}\sum_{t \in E^m} c_{k, \ell}^t\).

    We know that \(q_{k, \ell}^m = \frac{n^m_{k, \ell}}{N_{\max}^m}\). We also define the corruption on agent \(\ell\)'s rewards as \(C_{\ell}^m = \sum_{t \in E^m}\max_{k \in \mathcal{K}_{\ell}} |c_{k, \ell}^t|\), therefore we can conclude that \(\sum_{t \in E^m} \left|c_{k, \ell}^t\right| \leq C_{\ell}^m\). We choose a parameter \(\beta \geq 4e^{(-\lambda/16)}\), therefore \(n_{k, \ell}^m \geq \lambda \geq 16\ln{\left(4/\beta\right)}\), and so \(n_{k}^m \geq \lambda \geq 16\ln{\left(4/\beta\right)}\). Then we can rewrite the same bound as:
    \begin{align}
        \label{eqn:B_corr_1}
        \frac{B_{k}^m}{n_{k}^m}\leq 2\sum_{\ell \in \mathcal{L}_k}\frac{n^m_{k, \ell}}{n_k^m}\frac{C^m_\ell}{N^m_{\max}} + \sqrt{\frac{\ln{\frac{4}{\beta}}}{16n_{k}^m}}.
    \end{align}
    \eqref{eqn:B_corr_1} holds for \(-\frac{B_{k}^m}{n_{k, \ell}^m}\) with the same probability, Therefore we have:
    \begin{align}
        \label{eqn:B_1}
        Pr\left[\left|\frac{B_{k}^m}{n_{k}^m}\right| \geq 2\sum_{\ell \in \mathcal{L}_k}\frac{n^m_{k, \ell}}{n_k^m}\frac{C^m_\ell}{N^m_{\max}} + \sqrt{\frac{\ln{\frac{4}{\beta}}}{16n_{k}^m}}\right] \leq \frac{\beta}{2}.
    \end{align}


    \item
    \paragraph{Combining the two small probability bounds}Combining \eqref{eqn:A2} and \eqref{eqn:B}, we have:
    \begin{align*}
        Pr\left[\left|r_{k}^m - \mu_k\right| \geq 2\sum_{\ell \in \mathcal{L}_k}\frac{n^m_{k, \ell}}{n_k^m}\frac{C^m_\ell}{N^m_{\max}} + \sqrt{\frac{4\ln{\frac{4}{\beta}}}{n_{k}^m}}\right] \leq \beta.
    \end{align*}

    Then we set \(\beta = \delta/(2K\log{T})\), as this value satisfies \(\beta \geq 4e^{-\lambda/16}\), we have:
    \begin{align*}
        Pr\left[\left|r_{k}^m - \mu_k\right| \geq 2\sum_{\ell \in \mathcal{L}_k}\frac{n^m_{k, \ell}}{n_k^m}\frac{C^m_\ell}{N^m_{\max}} + \frac{1}{16\sqrt{\sum_{\ell \in \mathcal{L}_k}(\Delta^m_{k, \ell})^{-2}}}\right] \leq \delta/(2K\log{T}).
    \end{align*}
    \item
    \begin{claim}\label{cl:1}
        \begin{align}
            \Pr\left[\Tilde{n}_{k, \ell}^m \geq 2 \cdot n_{k, \ell}^m\right] \leq \beta
        \end{align}
    \end{claim}

    \begin{proof}
        We can again use a Hoeffding bound on the r.v. representing the actual number of pulls of arm \(k\) in epoch \(m\), which is: \(\tilde{n}_{k, \ell}^m \coloneqq \sum_{t \in E^m_\ell} Y_{k, \ell}^t\). The expected value of this r.v. is \(\mathbb{E}\left[\tilde{n}_{k, \ell}^m\right] = N_{\ell}^m\frac{n_{k}^m}{N_{\ell}^m} = {n_{k, l}^m}\). The probability that the r.v. is more than twice its expectation is at most: \(2\exp{\left(-\frac{2(n_{k, l}^m)^2}{3(N^m_{\max})^2}\right)} \leq 2\exp{\left(-\frac{2\lambda^2}{3T^2}\right)} \leq 4\exp{\left(\frac{-\lambda}{16}\right)}\leq \beta\).
    \end{proof}

    Therefore using a union bound, we have:
    \begin{align}\label{eq:lem2_2}
        \Pr\bigg[\forall k\in \mathcal{K}, m \in \{1, 2, \dots, M\}: & \left|r_{k}^m - \mu_k\right| \geq 2\sum_{\ell \in \mathcal{L}_k}\frac{n^m_{k, \ell}}{n_k^m}\frac{C^m_\ell}{N^m_{\max}} + \frac{1}{16\sqrt{\sum_{\ell \in \mathcal{L}_k}(\Delta^m_{k, \ell})^{-2}}} \\
        \text{and }                                                  & \Tilde{n}_{k, \ell}^m \geq 2 \cdot n_{k, \ell}^m \bigg] \leq \delta.
    \end{align}

    The term \(2\sum_{\ell \in \mathcal{L}_k}\frac{n^m_{k, \ell}}{n_k^m}\frac{C^m_\ell}{N^m_{\max}}\) is a weighted average of the epoch corruption of the agents in \(\mathcal{L}_k\), weighted based on \(n_{k, \ell}^m\) for every agent \(\ell\). This term can be upper bounded by the maximum term that is being averaged, \(2\max_{\ell \in \mathcal{L}}\frac{C^m_\ell}{N^m_{\max}}\).
    Also, as for every agent \(\ell\), \(\Delta_{k, \ell}^{m-1} \leq \Delta_{k, \max}^{m-1}\), we can replace \(\frac{1}{16\sqrt{\sum_{\ell \in \mathcal{L}_k}(\Delta^m_{k, \ell})^{-2}}}\) with \(\frac{\Delta_{k, \max}^{m-1}}{16}\). And this concludes the proof of Lemma~\ref{lem:4}.
\end{proof}


Now let us define \(D^m\) as:
\begin{equation}\label{eq:dm_d_a}
    D^m = 2\max_{\ell \in \mathcal{L}}\frac{C^m_\ell}{N^m_{\max}},
\end{equation}

\begin{lemma}
    Suppose that \(\mathcal{E}\) happens, then for all epochs \(m\):
    \label{lem:5}
    \begin{align}
        -D^m - \frac{\Delta^{m - 1}_{k_{*, \ell}, \max}}{8} \leq r_{*, \ell}^m - \mu_{*, \ell} \leq D^m.
    \end{align}
    where
\end{lemma}


\begin{proof}
    We know that \(r_{*, \ell}^m = \max_{k\in\mathcal{K}_\ell}{\{r_{k}^m - \frac{1}{16}\Delta_{k, \max}^{m - 1}\}}\) and therefore \(r_{*, \ell}^m \geq r_{k_{*, \ell}}^m - \frac{1}{16}\Delta_{k_{*, \ell}, \max}^{m - 1}\). Considering the lower bound implied by \(\mathcal{E}\) we have:
    \begin{align*}
        2\max_{\ell \in \mathcal{L}}\frac{C^m_\ell}{N^m_{\max}} - \frac{\Delta_{k_{*, \ell}, \max}^{m - 1}}{8} \leq r_{*, \ell}^m - \mu_{*, \ell},
    \end{align*}
    since \(\mathcal{L}_{k_{*, \ell}} \subseteq \{\ell\} + \mathcal{N}(\ell)\), we have \(C_{\mathcal{L}_{k_{*, \ell}}} \leq C_{\ell} + C_{\mathcal{N}(\ell)}\), therefore we can rewrite the inequality as:
    \begin{align*}
        -D^m - \frac{\Delta_{k_{*, \ell}, \max}^{m - 1}}{8} \leq r_{*, \ell}^m - \mu_{*, \ell},
    \end{align*}
    We also know that:
    \begin{align*}
        r_{*, \ell}^m & = \max_{k\in\mathcal{K}_\ell}{\{r_{k}^m - \frac{1}{16}\Delta_{k, \max}^{m - 1}\}}                                                                                                                         \\
                      & \leq \max_{k\in\mathcal{K}_\ell}{\{\frac{2}{L_{k_{*, \ell}}}\frac{C^m_{\mathcal{L}_{k_{*, \ell}}}}{N^m_{\max}}} + \frac{1}{16}\Delta_{k, \max}^{m - 1} + \mu_{k} - \frac{1}{16}\Delta_{k, \max}^{m - 1}\} \\
                      & \leq \mu_{*, \ell} + D_\ell^m.
    \end{align*}
    Therefore the lemma is proved.
\end{proof}

Then we define \(\rho^m\) as:
\begin{equation}\label{eq:rho_d}
    \rho^m = \sum_{s = 1}^{m}\frac{D^s}{8^{m - s}}.
\end{equation}

\begin{lemma}
    \label{lem:6}
    Suppose that \(\mathcal{E}\) happens, then for all epochs \(m\), arm \(k\), and agent \(\ell\):
    \begin{align}
        \Delta_{k, \ell}^m \leq 2(\Delta_{k, \ell} + 2^{-m} + \rho^m).
    \end{align}
\end{lemma}



\begin{proof}
    We prove this by induction on \(m\). For \(m = 1\), the claim is true for all \(k\) and \(\ell\), as \(\Delta_{k, \ell}^m \leq 1 \leq 2\cdot2^{-m}\).

    Suppose that the claim holds for \(m - 1\). Using Lemma~\ref{lem:5} and the definition  of the event \(\mathcal{E}\), we write:
    \begin{equation}
        % \resizebox{.94\linewidth}{!}{
        \begin{split}
            \quad r_{*, \ell}^m - r_{k, \ell}^m & = (r_{*, \ell}^m - \mu_{*,\ell}) + (\mu_{*,\ell} - \mu_k) + (\mu_k - r_{k, \ell}^m)                                                                      \\
                                                & \overset{(a)}\leq D^m + \Delta_{k, \ell} + D^m + \frac{\Delta^{m - 1}_{k, \max}}{16}                                                                     \\
                                                & \overset{(b)}\leq \Delta_{k, \ell} + 2D^m + \frac{1}{8}\left(\Delta_{k, \ell} + 2^{-(m-1)} + \sum_{s = 1}^{m-1}\frac{D^{s}_\ell}{8^{(m - 1) - s}}\right) \\
                                                & \leq 2\left(\Delta_{k, \ell} + 2^{-m} + \sum_{s = 1}^{m}\frac{D^{s}_\ell}{8^{m - s}}\right),
        \end{split}
        % }
    \end{equation}
    where inequality (a) holds because \((r_{*, \ell}^m - \mu_{*,\ell})\) is bound using Lemma~\ref{lem:5}, and \((\mu_k - r_{k, \ell}^m)\) is bound following the assumption of event \(\mathcal{E}\). Also, inequality (b) holds due to the induction's hypothesis.
    Therefore Lemma~\ref{lem:6} is proved.
\end{proof}


\begin{lemma}
    \label{lem:7}
    Suppose that \(\mathcal{E}\) happens, then for all epochs \(m\), arm \(k\), and agent \(\ell\):
    \begin{align}
        \Delta_{k, \ell}^m \geq \frac{1}{2} \Delta_{k, \ell} - 3\rho^m -\frac{3}{4}2^{-m}.
    \end{align}
\end{lemma}

\begin{proof}
    \begin{align*}
        \Delta_{k, \ell}^m  \geq r_{*, \ell}^m - r_{k, \ell}^m
         & \overset{(a)}\geq \left(\mu_{*, \ell} - D^m - \frac{\Delta^{m - 1}_{k_{*, \ell}, \max}}{8}\right) - \left(\mu_k + D^m + \frac{\Delta^{m - 1}_{k, \max}}{16}\right) \\
         & \overset{(b)}\geq \Delta_{k, \ell} - 2D^m - \left(\frac{3}{8}\rho^{m-1} + \frac{3}{8}2^{-(m - 1)} + \frac{3}{8}\Delta_{k, \ell}\right)                             \\
         & \geq \frac{1}{2} \Delta_{k, \ell} - 3\sum_{s = 1}^{m}\frac{D_{\ell}^{s}}{8^{m - s}} -\frac{3}{4}2^{-m}.
    \end{align*}
    where (a) holds because \(r_{*, \ell}^m\) can be bound using Lemma~\ref{lem:5}, and \(r_{k, \ell}^m\) is bound due to event \(\mathcal{E}\), and (b) is because of Lemma~\ref{lem:6}.
\end{proof}


\subsubsection{Proof for Theorem~\ref{theo:1}}

We decompose the total regret of each agent across epochs and within epochs, to the arms pulled. There are \(\tilde{n}^m_{k, \ell}\) pulls of arm \(k\) in epoch \(m\) for agent \(\ell\), each causing a regret of \((\mu_{*, \ell} - \mu_k)\). Thus the total regret of agent \(\ell\) can be written as:
\begin{align*}
    \sum_{m = 1}^{M}{\sum_{k \in \mathcal{K}_\ell}{(\mu_{*, \ell} - \mu_k)\tilde{n}^m_{k, \ell}}} & \overset{(a)}\leq 2\sum_{m = 1}^{M}{\sum_{k \in \mathcal{K}_\ell}{(\mu_{*, \ell} - \mu_k){n^m_{k, \ell}}}} \\
                                                                                                  & = 2\sum_{m = 1}^{M}{\sum_{k \in \mathcal{K}_\ell}{\Delta_{k, \ell}{n^m_{k, \ell}}}},
\end{align*}
where inequality (a) holds under event \(\mathcal{E}\) defined in~\eqref{eq:event-E_d}.

Fix an epoch \(m\), an agent \(\ell\) and an arm \(k\) and denote \(\mathcal{R}^m_{k, \ell} := \Delta_{k, \ell}{n^m_{k, \ell}}\) as the approximate regret for this \((m ,\ell, k)\) triad. Recall that \(n^m_{k, \ell} = \lambda(\Delta_{k, \ell}^{m-1})^{-2}\leq \lambda2^{2(m - 1)}\). Consider the three following cases:

\paragraph{Case 1} \(0 \leq \Delta_{k, \ell} \leq 4/2^{m}\).
In this case we can upper bound \(n_{k, \ell}^m \leq \frac{\lambda2^{2(m - 1)}}{L_k}\), which follows:
\begin{align*}
    \mathcal{R}_{k, \ell}^m \leq \frac{4\lambda}{L_k\Delta_{k, \ell}}.
\end{align*}

\paragraph{Case 2} \(\Delta_{k, \ell} > 4/2^{m}\) and \(\rho^m < \Delta_{k, \ell}/32\). In this case we can write:
\begin{align*}
    \Delta_{k, \ell}^{m-1} & \overset{(a)}\geq \frac{1}{2} \Delta_{k, \ell} - 3\rho^{m-1} -\frac{3}{4}2^{-(m-1)}                          \\
                           & \geq \Delta_{k, \ell} \left( \frac{1}{2} - \frac{3}{32} - \frac{3}{8} \right) = \frac{\Delta_{k, \ell}}{32},
\end{align*}
where inequality (a) holds for Lemma~\ref{lem:7}.

Therefore we can bound \(\mathcal{R}_{k, \ell}^m\) as:
\begin{align*}
    \mathcal{R}_{k, \ell}^m \leq \frac{2^{10}\lambda}{L_k\Delta_{k, \ell}}.
\end{align*}

\paragraph{Case 3} \(\Delta_{k, \ell} > 4/2^{m}\) and \(\rho^m \geq \Delta_{k, \ell}/32\). Therefore \(\Delta_{k, \ell} \leq 32 \rho^m\). Then:
\begin{align*}
    \mathcal{R}_{k, \ell}^m \leq {\lambda\Delta_{k, \ell}2^{2(m - 1)}} \leq {8\frac{\lambda}{L_k}\rho^{m-1}2^{2m}}.
\end{align*}
Combining the three cases, we have:
\begin{align*}
    \mathcal{R}_{k, \ell}^m \leq \frac{32^2\lambda}{L_k\Delta_{k, \ell}} + {8\frac{\lambda}{L_k}\rho^{m-1}2^{2m}}.
\end{align*}

Summing over all epochs, arms and agents, we can write the aggregated regret as:
\begin{equation}
    % \resizebox{.99\linewidth}{!}{
    \begin{split}
        2\sum_{k \in \mathcal{K}}\sum_{\ell \in \mathcal{L}_k} \sum_{m = 1}^{M} \mathcal{R}_{k, \ell}^m & \leq \sum_{k \in \mathcal{K}}\sum_{\ell \in \mathcal{L}_k}  \sum_{m = 1}^{M} \frac{2^{11}\lambda}{L_k\Delta_{k, \ell}} + \sum_{k \in \mathcal{K}}\sum_{\ell \in \mathcal{L}_k} \sum_{m = 1}^{M} {16\frac{\lambda}{L_k}\rho^{m-1}2^{2m}} \\
                                                                                                        & \leq 2^{11}\lambda\sum_{k \in \mathcal{K}}\sum_{\ell \in \mathcal{L}_k} \frac{\log{T}}{L_k\Delta_{k, \ell}} + 16\lambda\sum_{k \in \mathcal{K}}\sum_{\ell \in \mathcal{L}_k}\frac{1}{L_k}\sum_{m = 1}^{M} \rho^{m-1}2^{2m}.
    \end{split}
    % }
\end{equation}

Let us first bound \(\sum_{m = 1}^{M} \rho^{m-1}2^{2m}\):
\begin{equation}
    % \resizebox{.99\linewidth}{!}{
    \begin{split}
        \sum_{m = 1}^{M} \rho^{m-1}2^{2m} & \overset{\eqref{eq:rho_d}}= \sum_{m = 1}^{M} 2^{2m} \sum_{s = 1}^{m-1}\frac{D^{s}}{8^{m - s - 1}} = \sum_{s = 1}^{M - 1} D^s \sum_{m = s + 1}^{M} \frac{2^{2m}}{8^{m - 1 - s}} \\
                                          & \overset{\eqref{eq:dm_d_a}}= \sum_{s = 1}^{M - 1} {2\frac{\max_{\ell \in \mathcal{L}_k}C_{\ell}^s}{N_{\max}^s}} \sum_{m = s+1}^{M} \frac{2^{2m}}{8^{m - 1 - s}}                \\
                                          & \overset{(a)}\leq \sum_{s = 1}^{M - 1} {\frac{32\hat L}{\lambda}\max_{\ell \in \mathcal{L}_k}C_{\ell}^s} \sum_{m = s + 1}^{M} \frac{4^{m - 1 - s}}{8^{m - 1 - s}}              \\
                                          & \leq \frac{32\hat L}{\lambda} \max_{\ell \in \mathcal{L}_k}C_{\ell}^s,
    \end{split}
    % }
\end{equation}
where (a) is because \(N_{\max}^m \geq \frac{\lambda2^{-2(m - 1)}}{\hat L}\).

Therefore the second part of the aggregated regret can be written as:
\begin{equation}
    % \resizebox{.99\linewidth}{!}{
    \begin{split}
        16\lambda\sum_{k \in \mathcal{K}}\sum_{\ell \in \mathcal{L}_k}\frac{1}{L_k}\sum_{m = 1}^{M} \rho^{m-1}2^{2m} \leq  16\lambda\sum_{k \in \mathcal{K}}\sum_{\ell \in \mathcal{L}_k} \frac{1}{L_k} \frac{32\hat L}{\lambda} \max_{\ell \in \mathcal{L}_k}C_{\ell}^s
    \end{split}
    % }
\end{equation}

As \(\lambda = 1024\ln\left(\frac{8KL}{\delta}\log T\right)\), the total aggregated regret can be bounded as follows, with probability at least \(1 - \delta\).
\begin{align}
    O\left(\hat L\sum_{k \in \mathcal{K}}\sum_{\ell \in \mathcal{L}_k} \frac{\max_{\ell \in \mathcal{L}_k}C_{\ell}}{L_k}  + \log{\left(\frac{K}{\delta}\log{T}\right)}\sum_{k \in \mathcal{K}}\frac{\sum_{\ell \in \mathcal{L}_k}\left(\Delta_{k, \ell}\right)^{-1}}{L_{k}}\log{T}\right).
\end{align}
And as the communication broadcast is done at the end of each epoch, according to Lemma~\ref{lem:2_4} the communication cost is:
\begin{align}
    O\left(L\log\left(\frac{T}{\ln(\frac{8K}{\delta}\log T)}\right)\right).
\end{align}

\subsection{\lfbarbar Homogeneous case}\label{appendix:a_1_2}
In the homogeneous case, all agents have access to all arms. Therefore, at every epoch, \(r_{*, \ell_1}^m = r_{*, \ell_2}^m\) for every agent pair \(\ell_1\) and \(\ell_2\). Consequently, \(\Delta_{k, \ell_1}^m = \Delta_{k, \ell_2}^m\) and thus \(n_{k, \ell_1}^m = n_{k, \ell_2}^m\).

We can then rewrite \eqref{eq:lem2_2} and redefine the event \(\mathcal{E}\) as:
\begin{align}\label{eq:event-E_d_h}
    \mathcal{E} \coloneqq \left\{\forall k\in \mathcal{K}, \ell\in \mathcal{L}, m \in \{1, 2, \dots, M\} : \left|r_{k}^m - \mu_k\right| \geq \frac{2}{L}\sum_{\ell \in \mathcal{L}}\frac{C^m_\ell}{N^m_{\max}} + \frac{\Delta_{k, \max}^{m-1}}{16} \text{ and } \Tilde{n}_{k, \ell}^m \geq {2 n_{k, \ell}^m} \right\},
\end{align}

Subsequently, we define \(D^m\) as:
\begin{equation}\label{eq:dm_d_a_2}
    D^m = \frac{2}{L}\sum_{\ell \in \mathcal{L}}\frac{C^m_\ell}{N^m_{\max}}.
\end{equation}
Following the same proof as in Appendix~\ref{appendix:a_1}, we can upper bound the total regret as:
\begin{align}
    O\left(KC + \log{\left(\frac{K}{\delta}\log{T}\right)}\sum_{k \in \mathcal{K}}\frac{\sum_{\ell \in \mathcal{L}_k}\left(\Delta_{k, \ell}\right)^{-1}}{L_{k}}\log{T}\right).
\end{align}

\subsection{\lfbarbar tightness (Proof for Theorem~\ref{theo:2})}\label{appendix:a_2}
% \subsubsection{Proof for Theorem~\ref{theo:2}}
\begin{proof}

    Here we aim to give an example here that suffers the regret of \(\Omega\left(\sum_{\ell \in \mathcal{L}} \sum_{k \in \mathcal{K}_\ell} \frac{\hat L}{L_k}\max_{\ell \in \mathcal{L}_k}C_{\ell}\right)\). Consider the case where every arm is accessible by exactly \(L'\) agents. Among these arms only one has a expected reward of \(1\), let us call that arm \(1\). And others have an expected reward equal to \(0\). In this example we discuss the worst case that can lead to the mentioned lower bound.

    In the case without corruption, for each epoch \(m \geq 1\) and for any agent \(\ell \in \mathcal{L}_1\), we have \(\Delta^m_{1} = 2^{-m}\), as \(\Delta^m_{1} = \max{\{2^{-m}, r_{*}^m - r_{1}^m\}}\), and \(r_{*}^m = r_{1}^m\). For every other arm \(k \in \mathcal{K}_\ell\), \(\Delta_{k}^m = r^m_{*} = {1} - \frac{(1) - (1/16)^m}{15} \in [14/15, 15/16]\).
    Therefore, with no corruption, the \(m\)th epoch has length:
    \begin{align*}
        N^m_\ell
        = \sum_{k \in \mathcal{K}_\ell}\frac{n_{k}^m}{L_k}
        = \sum_{k \in \mathcal{K}_\ell}\frac{ \lambda(\Delta_{k, \ell}^{m - 1})^{-2}}{L_k}
        = \frac{\lambda}{L'}\left(2^{2(m-1)}+O\left(K_\ell\right)\right).
    \end{align*}

    Now consider a case where the rewards of arm 1 is only corrupted in every round of a certain epoch \(m\in\{1,2,\dots,M\}\). Therefore the total amount of corruption is equal to:
    \begin{align*}
        C = \sum_{\ell \in \mathcal{L}_1} C_\ell = \sum_{\ell \in \mathcal{L}_1} \frac{\lambda}{L'}\left(2^{2(m - 1)}+O\left(K_\ell\right)\right)
        = {\lambda}\left(2^{2(m - 1)}+ \sum_{\ell \in \mathcal{L}_1}O\left(K_\ell\right)\right)
    \end{align*}

    Note that the corruption is only affecting arm \(1\) in epoch \(m\), making every observed reward equal to 0. Therefore \(r^m_{*} \leq 0\) and all \(\Delta_{k}^m = 2^{-m}\). And therefore the length of the next epoch for agent \(\ell \in \mathcal{L}_1\) will be:
    \begin{align*}
        N^{m+1}_\ell = \lambda2^{2m}\sum_{k \in \mathcal{K}_\ell}\frac{1}{L'}
        % \approx C\frac{K_\ell}{L'} 
        = \Omega\left(\frac{CK_\ell}{L'}\right).
    \end{align*}

    Therefore in epoch \(m+1\), agent \(\ell \in \mathcal{L}'\) has at least \(\Omega\left(\frac{CK_\ell}{L'}\right)\) arm pulls, and every arm has an equal probability to be selected for each agent. Hence, with a probability of \(1 - (1 - \frac{1}{K})^L\) the best arm will not be assigned to any agents. This probability is high for some pairs of \(K\) and \(L\), for example, when \(K = 40\) and \(L = 100\), \(1 - (1 - \frac{1}{K})^L \geq 0.9\).
    In that case, we will have a regret of \(\Omega\left(\frac{CK}{L'}\right)\) for agent \(\ell\), and consequently a total regret of \(\Omega\left({CK}\right)\). In this case, as \(\hat L\) and \(L_k\) are equal to \(L'\) for all \(k \in \mathcal{K}\), and \(\max_{\ell \in \mathcal{L}} C_{\ell} = \frac{C}{L'}\), we have: \(\Omega\left(\sum_{\ell \in \mathcal{L}} \sum_{k \in \mathcal{K}_\ell} \frac{\hat L}{L_k}\max_{\ell \in \mathcal{L}_k}C_{\ell}\right) = \Omega\left(KC\right)\).

\end{proof}

% \section{\distbarbar}\label{appendix:b}
% \subsection{\distbarbar Regret Upper Bound}\label{appendix:b_1}
% \subsubsection{Lemmas for Proving Theorem~\ref{theo:3}}
% \begin{lemma}
% We can bound variable \(N_{\max}^m\) as:
%     \begin{align}
%        \lambda2^{2(m-1)} \leq N_{\max}^{m} \leq K\lambda2^{2(m-1)},
%     \end{align}
%     and the number of epochs \(M\) is at most \(\log{T}\).
% \end{lemma}


% \begin{proof}
%     For each agent \(\ell\), there exists an arm \(k_{\ell}^m\) achieving the reward \(r^m_{*, \ell}\) and fulfilling \(r^m_{*, \ell} - r^m_{k_{\ell}^m} \leq 0\). Therefore \(\Delta^m_{k_{\ell}^m, \ell} = 2^{-m}\). So we have:
%     \begin{align*}
%         N_\ell^{m + 1} \geq n^{m + 1}_{k_{\ell}^m, \ell} = \lambda\left(\Delta^m_{k_{\ell}^m, \ell}\right)^{-2} = \lambda2^{2m}.
%     \end{align*}
%     On the other hand, since that \(\Delta_{k, \ell}^{m} \geq 2^{-m}\), so for each \(k\) we have \(n^m_{k, \ell} \leq \lambda2^{2m}\). Hence, the lemma is proved. The bound on \(m\) follows the lower bound on \(N_\ell^{m}\).

% \end{proof}

% We define an event \(\mathcal{E}\) such as:
%  \begin{align}\label{eq:event-E_d}
%         \mathcal{E} \coloneqq \left\{\forall k\in \mathcal{K}, \ell\in \mathcal{L}_k, m \in \{1, 2, \dots, M\} : \left|r_{k}^m - \mu_k\right| \geq \frac{2}{L_k}\frac{C^m_{\mathcal{L}_k}}{N^m_{\max}} + \frac{\Delta_{k, \max}^{m-1}}{16} \text{ and } \Tilde{n}_{k, \ell}^m \geq {2 n_{k, \ell}^m} \right\},
%     \end{align}
% where \(C_{\mathcal{L}_k}^m\) is the total corruption on agents in set \(\mathcal{L}_k\) in epoch \(m\), and \(\Tilde{n}_{k, \ell}^m\) is the actual number of pulls of arm \(k\) by agent \(\ell\) in epoch \(m\).

% % such that \(C = \sum_{\ell \in \mathcal{L}} \sum_{m = 1}^M C_\ell^m\)

% \begin{lemma}\label{lem:4}
%     It holds that:
%     \begin{align}
%         \Pr[\mathcal{E}] \geq 1 - \delta.
%     \end{align}
% \end{lemma}


% \begin{proof}
%     % \(\beta \geq 4e^{-\frac{\lambda}{16L}}\), where \(L\) is the total number of agents.
% % For any fixed \(\ell \in \mathcal{L}\), \(k \in \mathcal{K}_{\ell}\), and \(m\) we have:
%     \item
%     \paragraph{Decomposing \(\pmb{r_{k}^m}\)}For this proof, we condition on all random variables before some fixed epoch \(m\), so that \(n^m_{k, \ell}\) , \(N_{\ell}^m\) and \(T_{\ell}^{m-1}\) are deterministic quantities. At each step in this epoch, agent \(\ell\) picks arm \(k\) with probability \(q_{k, \ell}^m \coloneqq \frac{n^m_{k, \ell}}{N_{\max}^m}\). Let \(Y_{k, \ell}^t\) be an indicator for arm \(k\) being pulled in step \(t\) by agent \(\ell\). Let \(R_{k, \ell}^t\) be the stochastic reward of arm \(k\) on step \(t\) for agent \(\ell\). and \(c^t_{k, \ell} \coloneqq \tilde{R}_{k, \ell}^t - R_{k, \ell}^t\) be the corruption added to arm \(k\) by the adversary in step \(t\) for agent \(\ell\). Note that \(c^t_{k, \ell}\) may depend on all the stochastic rewards up to (and including) round \(t\), and also on all previous choices of the algorithm (though not the choice at step \(t\). Finally, if we denote \(E^m = \{T^{m-1} + 1, . . . , T^{m}\}\) to be the \(N_{\max}^{m}\) timesteps in epoch \(m\), then we define a random variable \(r_{k, \ell}^m\) as follows:
%     \begin{equation}
%         r_{k, \ell}^m = \frac{1}{n_{k, \ell}^m}\sum_{t \in E^m}Y_{k, \ell}^t(R_{k, \ell}^t + c_{k, \ell}^t).
%     \end{equation}
%     Let us break this sum into two:
%     \begin{align*}
%         A_{k, \ell}^m & = \sum_{t \in E^m}Y_{k, \ell}^tR_{k, \ell}^t \\
%         B_{k, \ell}^m & = \sum_{t \in E^m}Y_{k, \ell}^tc_{k, \ell}^t.
%     \end{align*}

%     \item
%     \paragraph{Bounding the first and the second part} To \textbf{bound the first part}, we first note that:
%     \begin{align*}
%         \mathbb{E}\left[A_{k, \ell}^m\right] = N^m_{\max}.\left(q_{k, \ell}^m\mu_k\right) = n_{k, \ell}^m\mu_k.
%     \end{align*}

%     Therefore, according to the Chernoff-Hoeffding bound \cite{dubhashi2009concentration}, for \(\beta \leq 1\) we have:
%     \begin{align}
%         \label{eqn:A2}
%         Pr\left[\left|\frac{A_{k, \ell}^m}{n_{k, \ell}^m} - \mu_k\right| \geq \sqrt{\frac{3\ln{\frac{4}{\beta}}}{n_{k, \ell}^m}}\right] \leq \frac{\beta}{2}.
%     \end{align}


%     Next, we aim to \textbf{bound the second part}. To this end, we define the sequence of r.v.s, \(\{X_t\}_{t=1}^T\) for agent \(\ell\), where \(X_t = \left(Y_{k, \ell}^t - q_{k, \ell}^m\right)\cdot c_{k, \ell}^t\) for all \(t\). Then \(\{X_t\}_{t=1}^T\) is a martingale sequence with respect to the filtration \(\{\mathcal{F}_t\}_{t=1}^T\) generated by r.v.s \(\{Y_{k, h}^s\}_{h \in \mathcal{L}, k \in \mathcal{K}_h, s \leq t}\) and \(\{R_{k, h}^s\}_{h \in \mathcal{L}, k \in \mathcal{K}_h, s \leq t}\). The corruption \(c_{k, \ell}^m\) becomes deterministic conditioned on \(\mathcal{F}_{t-1}\), and since \(\mathbb{E}\left[Y_{k, \ell}^t | \mathcal{F}_{t-1}\right] = q_{k, \ell}^m\), we have:
%     \begin{align*}
%         \mathbb{E}\left[X_t | \mathcal{F}_{t-1}\right] = \mathbb{E}\left[Y_{k, \ell}^t - q_{k, \ell}^m | \mathcal{F}_{t-1}\right]\cdot c_{k, \ell}^t = 0.
%     \end{align*}

%     As \(\left|X_t\right| \leq 1\), using a Freedman-type concentration inequality introduced in \citeauthor{beygelzimer2011contextual}, the predictive quadratic variation of this martingale can be bounded as:
%     \begin{gather*}
%         \Pr\left[\sum_{t\in E^m} X_t \geq V + \ln \frac{4}{\beta}\right] \leq \frac{\beta}{4},
%     \end{gather*}
%     where
%     \begin{align*}
%         V = & \sum_{t \in E^m}\mathbb{E}\left[X_t^2 | \mathcal{F}_{t-1}\right] \leq \sum_{t \in E^m} \left|c_{k, \ell}^t\right|\text{Var}\left(Y_{k, \ell}^t\right) \leq q_{k, \ell}^m\sum_{t \in E^m} \left|c_{k, \ell}^t\right|.
%     \end{align*}
%     Therefore, we obtain that with a probability of \(1 - \frac{\beta}{4}\):
%     \begin{align*}
%         \frac{B_{k, \ell}^m}{n_{k, \ell}^m} & \overset{(a)}\leq \frac{q_{k, \ell}^m}{n_{k, \ell}^m}\sum_{t \in E^m} c_{k, \ell}^t + \frac{1}{n_{k, \ell}^m} \left(V + \ln{\frac{4}{\beta}}\right) \\
%         & \leq 2\frac{q_{k, \ell}^m}{n_{k, \ell}^m}\sum_{t \in E^m} \left|c_{k, \ell}^t\right| + \frac{1}{n_{k, \ell}^m} \ln{\frac{4}{\beta}},
%     \end{align*}
%     where (a) is because \(\sum_{t \in E^m}X_t = \sum_{t \in E^m}(Y_{k, \ell}^t - q_{k, \ell}^m)\cdot c_{k, \ell}^t = B_{k,\ell}^m - {q_{k, \ell}^m}\sum_{t \in E^m} c_{k, \ell}^t\). 

%     We know that \(q_{k, \ell}^m = \frac{n^m_{k, \ell}}{N_{\max}^m}\). We also define the corruption on agent \(\ell\)'s rewards as \(C_{\ell}^m = \sum_{t \in E^m}\max_{k \in \mathcal{K}_{\ell}} |c_{k, \ell}^t|\), therefore we can conclude that \(\sum_{t \in E^m} \left|c_{k, \ell}^t\right| \leq C_{\ell}^m\). We choose a parameter \(\beta \geq 4e^{(-\lambda/16L)}\), therefore \(n_{k, \ell}^m \geq \lambda \geq 16\ln{\left(4/\beta\right)}{L}\). Then we can rewrite the same bound as:
%     \begin{align}
%     \label{eqn:B_corr}
%         \frac{B_{k, \ell}^m}{n_{k, \ell}^m}\leq 2\frac{C^m_\ell}{N^m_{\max}} + \sqrt{\frac{\ln{\frac{4}{\beta}}}{16n_{k, \ell}^m}}.
%     \end{align}
%     \eqref{eqn:B_corr} holds for \(-\frac{B_{k, \ell}^m}{n_{k, \ell}^m}\) with the same probability, Therefore we have:
%     \begin{align}
%         \label{eqn:B}
%         Pr\left[\left|\frac{B_{k, \ell}^m}{n_{k, \ell}^m}\right| \geq 2\frac{C^m_\ell}{N^m_{\max}} + \sqrt{\frac{\ln{\frac{4}{\beta}}}{16n_{k, \ell}^m}}\right] \leq \frac{\beta}{2}.
%     \end{align}

%     \item
%     \paragraph{Combining the two small probability bounds}Combining \eqref{eqn:A2} and \eqref{eqn:B}, we have:
%     \begin{align*}
%         Pr\left[\left|r_{k, \ell}^m - \mu_k\right| \geq 2\frac{C^m_\ell}{N^m_{\max}} + \sqrt{\frac{4\ln{\frac{4}{\beta}}}{n_{k, \ell}^m}}\right] \leq \beta.
%     \end{align*}
%     Now we use union bound to bound \(r_{k}^m = \frac{1}{L_k}\sum_{\ell \in \mathcal{L}_k}r_{k, \ell}^m\)
%     \begin{align*}
%         Pr\left[\left|r_{k}^m - \mu_k\right| \geq \frac{2}{L_k}\frac{\sum_{\ell \in \mathcal{L}_k}C^m_\ell}{N^m_{\max}} + \frac{1}{L_k}\sum_{\ell \in \mathcal{L}_k}\sqrt{\frac{4\ln{\frac{4}{\beta}}}{n_{k, \ell}^m}}\right] \leq L\beta.
%     \end{align*}
%     Then we set \(\beta = \delta/(2KL\log{T})\), as this value satisfies \(\beta \geq 4e^{-\lambda/16L}\), we have:
%     \begin{align*}
%         Pr\left[\left|r_{k}^m - \mu_k\right| \geq \frac{2}{L_k}\frac{C^m_{\mathcal{L}_k}}{N^m_{\max}} + \frac{1}{L_k}\sum_{\ell \in \mathcal{L}_k}\frac{\Delta_{k, \ell}^m}{16}\right] \leq \delta/(2K\log{T}).
%     \end{align*}

%     \begin{align*}
%         Pr\left[\left|r_{k}^m - \mu_k\right| \geq 2\sum_{\ell \in \mathcal{L}_k}\frac{n^m_{k, \ell}}{n_k^m}\frac{C^m_\ell}{N^m_{\max}} + \frac{\Delta_{k, \max}^m}{16}\right] \leq \delta/(2K\log{T}).
%     \end{align*}
%     \item
%     \begin{claim}
%     \begin{align}
%         \Pr\left[\Tilde{n}_{k, \ell}^m \geq 2 \cdot n_{k, \ell}^m\right] \leq \beta
%     \end{align}
%     \end{claim}

%     \begin{proof}
%         Again, we can use a Chernoff-Hoeffding bound on the r.v. representing the actual number of pulls of arm \(k\) by agent \(\ell\) in eopch \(m\), which is: \(\tilde{n}_{k, \ell}^m \coloneqq \sum_{t \in E^m_\ell} Y_{k, \ell}^t\). The expected value of this r.v. is \(\mathbb{E}\left[\tilde{n}_{k, \ell}^m\right] = {n_{k, \ell}^m}\). The probability that the r.v. is more than twice its expectation is at most: \(2\exp{\left(-\frac{n_{k, \ell}^m}{3}\right)} \leq 2\exp{\left(-\frac{\lambda}{3}\right)} \leq 4\exp{\left(\frac{-\lambda}{16}\right)} \leq \beta\).
%     \end{proof}

%     Therefore using a union bound, we have:
%     \begin{align*}
%         \Pr\bigg[ & \forall k\in \mathcal{K}, m \in \{1, 2, \dots, M\}: \left|r_{k}^m - \mu_k\right| \geq 2\max_{\ell \in \mathcal{L}_k}\frac{C^m_\ell}{N^m_{\max}} + \frac{\Delta_{k, \max}^m}{16} \text{ and } \Tilde{n}_{k, \ell}^m \geq 2 \cdot n_{k, \ell}^m \bigg] \leq \delta.
%     \end{align*}

% \end{proof}


%     Therefore using a union bound, we have:
%     \begin{align*}
%         \Pr\bigg[ & \forall k\in \mathcal{K}, m \in \{1, 2, \dots, M\}: \left|r_{k}^m - \mu_k\right| \geq \frac{2}{L_k}\frac{C^m_{\mathcal{L}_k}}{N^m_{\max}} + \frac{1}{16}\sum_{\ell \in \mathcal{L}_k}\Delta_{k, \ell}^{m-1} \text{ and } \Tilde{n}_{k, \ell}^m \geq 2 \cdot n_{k, \ell}^m \bigg] \leq \delta.
%     \end{align*}

%     Also, as for every agent \(l\), \(\Delta_{k, \ell}^{m-1} \leq \Delta_{k, \max}^{m-1}\), we can replace \(\frac{1}{16}\sum_{\ell \in \mathcal{L}_k}\Delta_{k, \ell}^{m-1}\) with \(\frac{\Delta_{k, \max}^{m-1}}{16}\). And this concludes the proof of Lemma~\ref{lem:4}.
% \end{proof}

% Now let us define \(D^m_\ell\) as:
% \begin{equation}\label{eq:dm_d}
%     D^m_\ell = \frac{2}{L_{\min, \ell}} \frac{C_\ell^m + C_{\mathcal{N}_\ell}^m}{N^m_{\max}},
% \end{equation}
% where \(L_{\min, \ell}\) is the minimum number of agents with access to any of agent \(\ell\)'s arms, \(\mathcal{N}(\ell)\) is the set of agents that have mutual access to at least one arm with agent \(\ell\), and finally \(C_{\mathcal{N}(\ell)}\) is the corruption on the rewards of arms in \(\mathcal{N}(\ell)\).
% % \textbf{Lemma 5.}
% \begin{lemma}
%     Suppose that \(\mathcal{E}\) happens, then for all epochs \(m\) and every agent \(\ell\):
%     \label{lem:5}
%     \begin{align}
%         -D^m_\ell - \frac{\Delta^{m - 1}_{k_{*, \ell}, \max}}{8} \leq r_{*, \ell}^m - \mu_{*, \ell} \leq D^m_\ell.
%     \end{align}
%     where 
% \end{lemma}


% \begin{proof}
%     We know that \(r_{*, \ell}^m = \max_{k\in\mathcal{K}_\ell}{\{r_{k}^m - \frac{1}{16}\Delta_{k, \max}^{m - 1}\}}\) and therefore \(r_{*, \ell}^m \geq r_{k_{*, \ell}}^m - \frac{1}{16}\Delta_{k_{*, \ell}, \max}^{m - 1}\). Considering the lower bound implied by \(\mathcal{E}\) we have:
%     \begin{align*}
%         -\frac{2}{L_{k_{*, \ell}}}\frac{C^m_{\mathcal{L}_{k_{*, \ell}}}}{N^m_{\max}} - \frac{\Delta_{k_{*, \ell}, \max}^{m - 1}}{8} \leq r_{*, \ell}^m - \mu_{*, \ell},
%     \end{align*}
%     since \(\mathcal{L}_{k_{*, \ell}} \subseteq \{\ell\} + \mathcal{N}(\ell)\), we have \(C_{\mathcal{L}_{k_{*, \ell}}} \leq C_{\ell} + C_{\mathcal{N}(\ell)}\), therefore we can rewrite the inequality as:
%     \begin{align*}
%         -D^m_\ell - \frac{\Delta_{k_{*, \ell}, \max}^{m - 1}}{8} \leq r_{*, \ell}^m - \mu_{*, \ell},
%     \end{align*}
%     We also know that:
%     \begin{align*}
%         r_{*, \ell}^m & = \max_{k\in\mathcal{K}_\ell}{\{r_{k}^m - \frac{1}{16}\Delta_{k, \max}^{m - 1}\}}\\
%         & \leq \max_{k\in\mathcal{K}_\ell}{\{\frac{2}{L_{k_{*, \ell}}}\frac{C^m_{\mathcal{L}_{k_{*, \ell}}}}{N^m_{\max}}} + \frac{1}{16}\Delta_{k, \max}^{m - 1} + \mu_{k} - \frac{1}{16}\Delta_{k, \max}^{m - 1}\}\\
%         & \leq \mu_{*, \ell} + D_\ell^m.
%     \end{align*}
%     Therefore the lemma is proved.
% \end{proof}

% Then we define \(\rho^m_\ell\) as:
% \begin{equation}\label{eq:rho_d}
%     \rho^m_\ell = \sum_{s = 1}^{m}\frac{D^s_\ell}{8^{m - s}}.
% \end{equation}

% \begin{lemma}
%     \label{lem:6}
%     Suppose that \(\mathcal{E}\) happens, then for all epochs \(m\), arm \(k\), and agent \(\ell\):
%     \begin{align}
%         \Delta_{k, \ell}^m \leq 2(\Delta_{k, \ell} + 2^{-m} + \rho^m_{\ell}).
%     \end{align}
% \end{lemma}



% \begin{proof}
%     We prove this by induction on \(m\). For \(m = 1\), the claim is true for all \(k\) and \(\ell\), as \(\Delta_{k, \ell}^m \leq 1 \leq 2\cdot2^{-m}\).

%     Suppose that the claim holds for \(m - 1\). Using Lemma~\ref{lem:5} and the definition  of the event \(\mathcal{E}\), we write:
%     \begin{equation}
%         % \resizebox{.94\linewidth}{!}{
%         \begin{split}
%              \quad r_{*, \ell}^m - r_{k, \ell}^m &= (r_{*, \ell}^m - \mu_{*,\ell}) + (\mu_{*,\ell} - \mu_k) + (\mu_k - r_{k, \ell}^m)\\
%              & \overset{(a)}\leq D^m_\ell + \Delta_{k, \ell} + D^m_\ell + \frac{\Delta^{m - 1}_{k, \max}}{16}\\
%              & \overset{(b)}\leq \Delta_{k, \ell} + 2D^m_\ell + \frac{1}{8}\left(\Delta_{k, \ell} + 2^{-(m-1)} + \sum_{s = 1}^{m-1}\frac{D^{s}_\ell}{8^{(m - 1) - s}}\right) \\
%              & \leq 2\left(\Delta_{k, \ell} + 2^{-m} + \sum_{s = 1}^{m}\frac{D^{s}_\ell}{8^{m - s}}\right),
%         \end{split}
%         % }
%     \end{equation}
%     where inequality (a) holds because \((r_{*, \ell}^m - \mu_{*,\ell})\) is bound using Lemma~\ref{lem:5}, and \((\mu_k - r_{k, \ell}^m)\) is bound following the assumption of event \(\mathcal{E}\). Also, inequality (b) holds due to the induction's hypothesis.
%     Therefore Lemma~\ref{lem:6} is proved.
% \end{proof}


% \begin{lemma}
%     \label{lem:7}
%     Suppose that \(\mathcal{E}\) happens, then for all epochs \(m\), arm \(k\), and agent \(\ell\):
%     \begin{align}
%         \Delta_{k, \ell}^m \geq \frac{1}{2} \Delta_{k, \ell} - 3\rho^m_\ell -\frac{3}{4}2^{-m}.
%     \end{align}
% \end{lemma}

% \begin{proof}
%     \begin{align*}
%         \Delta_{k, \ell}^m  \geq r_{*, \ell}^m - r_{k, \ell}^m
%          & \overset{(a)}\geq \left(\mu_{*, \ell} - D^m_\ell - \frac{\Delta^{m - 1}_{k_{*, \ell}, \max}}{8}\right) - \left(\mu_k + D^m_\ell + \frac{\Delta^{m - 1}_{k, \max}}{16}\right) \\
%          & \overset{(b)}\geq \Delta_{k, \ell} - 2D^m_\ell - \left(\frac{3}{8}\rho_{\ell}^{m-1} + \frac{3}{8}2^{-(m - 1)} + \frac{3}{8}\Delta_{k, \ell}\right)\\
%          & \geq \frac{1}{2} \Delta_{k, \ell} - 3\sum_{s = 1}^{m}\frac{D_{\ell}^{s}}{8^{m - s}} -\frac{3}{4}2^{-m}.
%     \end{align*}
%     where (a) holds because \(r_{*, \ell}^m\) can be bound using Lemma~\ref{lem:5}, and \(r_{k, \ell}^m\) is bound due to event \(\mathcal{E}\), and (b) is because of Lemma~\ref{lem:6}.
% \end{proof}

% \subsubsection{Proof for Theorem~\ref{theo:3}}
% We decompose the total regret of each agent across epochs and within epochs, to the arms pulled. There are \(\tilde{n}^m_{k, \ell}\) pulls of arm \(k\) in epoch \(m\) for agent \(\ell\), each causing a regret of \((\mu_{*, \ell} - \mu_k)\). Thus the total regret of agent \(\ell\) can be written as:
% \begin{align*}
%     \sum_{m = 1}^{M}{\sum_{k \in \mathcal{K}_\ell}{(\mu_{*, \ell} - \mu_k)\tilde{n}^m_{k, \ell}}} & \overset{(a)}\leq 2\sum_{m = 1}^{M}{\sum_{k \in \mathcal{K}_\ell}{(\mu_{*, \ell} - \mu_k){n^m_{k, \ell}}}} \\
%     & = 2\sum_{m = 1}^{M}{\sum_{k \in \mathcal{K}_\ell}{\Delta_{k, \ell}{n^m_{k, \ell}}}},
% \end{align*}
% where inequality (a) holds under event \(\mathcal{E}\) defined in~\eqref{eq:event-E_d}.

% Fix an epoch \(m\), an agent \(\ell\) and an arm \(k\) and denote \(\mathcal{R}^m_{k, \ell} := \Delta_{k, \ell}{n^m_{k, \ell}}\) as the approximate regret for this \((m ,\ell, k)\) triad. Recall that \(n^m_{k, \ell} = \lambda(\Delta_{k, \ell}^{m-1})^{-2}\leq \lambda2^{2(m - 1)}\). Consider the three following cases:

% \paragraph{Case 1} \(0 \leq \Delta_{k, \ell} \leq 4/2^{m}\). 
% In this case we can upper bound \(n_{k, \ell}^m \leq \frac{\lambda2^{2(m - 1)}}{L_k}\), which follows:
% \begin{align*}
%     \mathcal{R}_{k, \ell}^m \leq \frac{4\lambda}{\Delta_{k, \ell}}.
% \end{align*}

% \paragraph{Case 2} \(\Delta_{k, \ell} > 4/2^{m}\) and \(\rho_{\ell}^m < \Delta_{k, \ell}/32\). In this case we can write:
% \begin{align*}
%     \Delta_{k, \ell}^{m-1} & \overset{(a)}\geq \frac{1}{2} \Delta_{k, \ell} - 3\rho^{m-1}_{\ell} -\frac{3}{4}2^{-(m-1)}\\
%     & \geq \Delta_{k, \ell} \left( \frac{1}{2} - \frac{3}{32} - \frac{3}{8} \right) = \frac{\Delta_{k, \ell}}{32},
% \end{align*}
% where inequality (a) holds for Lemma~\ref{lem:7}.

% Therefore we can bound \(\mathcal{R}_{k, \ell}^m\) as:
% \begin{align*}
%     \mathcal{R}_{k, \ell}^m \leq \frac{2^{10}\lambda}{\Delta_{k, \ell}}.
% \end{align*}

% \paragraph{Case 3} \(\Delta_{k, \ell} > 4/2^{m}\) and \(\rho_{\ell}^m \geq \Delta_{k, \ell}/32\). Therefore \(\Delta_{k, \ell} \leq 32 \rho_{\ell}^m\). Then:
% \begin{align*}
%     \mathcal{R}_{k, \ell}^m \leq {\lambda\Delta_{k, \ell}2^{2(m - 1)}} \leq {8\lambda\rho_{\ell}^{m-1}2^{2m}}.
% \end{align*}
% Combining the three cases, we have:
% \begin{align*}
%     \mathcal{R}_{k, \ell}^m \leq \frac{32^2\lambda}{\Delta_{k, \ell}} + {8\lambda\rho_{\ell}^{m-1}2^{2m}}.
% \end{align*}

% Summing over all epochs, arms and agents, we can write the aggregated regret as:
% \begin{equation}
%     % \resizebox{.99\linewidth}{!}{
%     \begin{split}
%         2\sum_{\ell \in \mathcal{L}} \sum_{k \in \mathcal{K}_\ell} \sum_{m = 1}^{M} \mathcal{R}_{k, \ell}^m & \leq \sum_{\ell \in \mathcal{L}} \sum_{k \in \mathcal{K}_\ell} \sum_{m = 1}^{M} \frac{2^{11}\lambda}{\Delta_{k, \ell}} + \sum_{\ell \in \mathcal{L}} \sum_{k \in \mathcal{K}_\ell} \sum_{m = 1}^{M} {16\lambda\rho_{\ell}^{m-1}2^{2m}} \\
%         & \leq 2^{11}\lambda\sum_{\ell \in \mathcal{L}} \sum_{k \in \mathcal{K}_\ell} \frac{\log{T}}{\Delta_{k, \ell}} + 16\lambda\sum_{\ell \in \mathcal{L}} \sum_{k \in \mathcal{K}_\ell}\sum_{m = 1}^{M} \rho_{\ell}^{m-1}2^{2m}.
%     \end{split}
%     % }
% \end{equation}

% Let us first bound \(\sum_{m = 1}^{M} \rho_{\ell}^{m-1}2^{2m}\):
% \begin{equation}
%     % \resizebox{.99\linewidth}{!}{
%     \begin{split}
%         \sum_{m = 1}^{M} \rho_{\ell}^{m-1}2^{2m} & \overset{\eqref{eq:rho_d}}= \sum_{m = 1}^{M} 2^{2m} \sum_{s = 1}^{m-1}\frac{D_{\ell}^{s}}{8^{m - s - 1}} = \sum_{s = 1}^{M - 1} D_{\ell}^s \sum_{m = s + 1}^{M} \frac{2^{2m}}{8^{m - 1 - s}} \\
%          & \overset{\eqref{eq:dm_d}}= \sum_{s = 1}^{M - 1} {\frac{2}{L_{\min, \ell}}\frac{C_{\ell}^s + C_{\mathcal{N}(\ell)}^s}{N_{\max}^s}} \sum_{m = s+1}^{M} \frac{2^{2m}}{8^{m - 1 - s}}\\
%          & \overset{(a)}\leq \sum_{s = 1}^{M - 1} {\frac{32}{\lambda L_{\min, \ell}}(C_{\ell}^s + C_{\mathcal{N}(\ell)}^s)} \sum_{m = s + 1}^{M} \frac{4^{m - 1 - s}}{8^{m - 1 - s}}    \\
%          & \leq \frac{32}{\lambda L_{\min, \ell}} (C_{\ell} + C_{\mathcal{N}(\ell)}),
%     \end{split}
%     % }
% \end{equation}
% where (a) is because \(N_{\max}^m \geq \frac{\lambda2^{-2(m - 1)}}{\hat L}\).

% Therefore the second part of the aggregated regret can be written as:
% \begin{equation}
%     % \resizebox{.99\linewidth}{!}{
%     \begin{split}
%         16\lambda\sum_{\ell \in \mathcal{L}} \sum_{k \in \mathcal{K}_\ell}\sum_{m = 1}^{M} \rho_{\ell}^{m-1}2^{2m} \leq  16\lambda\sum_{\ell \in \mathcal{L}} \sum_{k \in \mathcal{K}_\ell} \frac{32}{\lambda L_{\min, \ell}} (C_{\ell} + C_{\mathcal{N}(\ell)}) \leq 2^9\sum_{\ell \in \mathcal{L}}\frac{K_\ell}{L_{\min, \ell}}(C_{\ell} + C_{\mathcal{N}(\ell)}).
%     \end{split}
%     % }
% \end{equation}

% As \(\lambda = 1024\ln\left(\frac{8KL}{\delta}\log T\right)\), the total aggregated regret can be bounded as follows, with probability at least \(1 - \delta\).
% \begin{align}
%     O\left(\sum_{\ell \in \mathcal{L}}\frac{K_\ell}{L_{\min, \ell}}(C_{\ell} + C_{\mathcal{N}(\ell)}) + \frac{1}{L}\log{\left(\frac{KL}{\delta}\log{T}\right)}\sum_{\ell \in \mathcal{L}} \sum_{k \in \mathcal{K}_\ell} \frac{\log{T}}{\Delta_{k, \ell}}\right).
% \end{align}


\section{\distbarbar}
\subsection{\distbarbar Regret Upper Bound}\label{appendix:b_1}
\subsubsection{Lemmas for Proving Theorem~\ref{theo:3}}
\begin{lemma}
    We can bound variable \(N_{\max}^m\) as:
    \begin{align}
        \frac{\lambda2^{2(m-1)}}{\hat L} \leq N_{\max}^{m} \leq K\lambda2^{2(m-1)},
    \end{align}
    where \(\hat L = \min_{\ell \in \mathcal{L}}\max_{k \in \mathcal{K}_{\ell}}{L_{k}}\). Also, the number of epochs \(M\) is:
    \[
        M = O\left(\log(\frac{T}{\lambda})\right),
    \]
    which is at most \(O(\log(T))\).
\end{lemma}


\begin{proof}
    For each agent \(\ell\), there exists an arm \(k_{\ell}^m\) achieving the reward \(r^m_{*, \ell}\) and fulfilling \(r^m_{*, \ell} - r^m_{k_{\ell}^m} \leq 0\). Therefore \(\Delta^m_{k_{\ell}^m, \ell} = 2^{-m}\). So we have:
    \begin{align*}
        N_\ell^{m + 1} \geq {n^{m + 1}_{k_{\ell}^m, \ell}} \geq\frac{\lambda\left(\Delta^m_{k_{\ell}^m, \ell}\right)^{-2}}{\max_{k \in \mathcal{K}_{\ell}}{L_{k}}} = \frac{\lambda2^{2m}}{\max_{k \in \mathcal{K}_{\ell}}{L_{k}}}.
    \end{align*}
    On the other hand, since that \(\Delta_{k, \ell}^{m} \geq 2^{-m}\), so for each \(k\) we have \(n^m_{k, \ell} \leq \frac{\lambda2^{2m}}{L_k}\). Hence, the lemma is proved. The bound on \(M\) follows the lower bound on \(N_\ell^{m}\).

\end{proof}

We define an event \(\mathcal{E}\) such as:
\begin{align}\label{eq:event-E_d}
    \mathcal{E} \coloneqq \left\{\forall k\in \mathcal{K}, \ell\in \mathcal{L}_k, m \in \{1, 2, \dots, M\} : \left|r_{k}^m - \mu_k\right| \geq 2\frac{\max_{\ell \in \mathcal{L}_k}C^m_{\ell}}{N^m_{\max}} + \frac{\Delta_{k, \max}^{m-1}}{16} \text{ and } \Tilde{n}_{k, \ell}^m \geq {2 n_{k, \ell}^m} \right\},
\end{align}
where \(C_{\ell}^m\) is the total corruption on agent \(\ell\) in epoch \(m\), and \(\Tilde{n}_{k, \ell}^m\) is the actual number of pulls of arm \(k\) by agent \(\ell\) in epoch \(m\).

% such that \(C = \sum_{\ell \in \mathcal{L}} \sum_{m = 1}^M C_\ell^m\)

\begin{lemma}\label{lem:4}
    It holds that:
    \begin{align}
        \Pr[\mathcal{E}] \geq 1 - \delta.
    \end{align}
\end{lemma}


\begin{proof}
    % \(\beta \geq 4e^{-\frac{\lambda}{16L}}\), where \(L\) is the total number of agents.
    % For any fixed \(\ell \in \mathcal{L}\), \(k \in \mathcal{K}_{\ell}\), and \(m\) we have:
    \item
    \paragraph{Decomposing \(\pmb{r_{k}^m}\)}For this proof, we condition on all random variables before some fixed epoch \(m\), so that \(n^m_{k, \ell}\) , \(N_{\ell}^m\) and \(T_{\ell}^{m-1}\) are deterministic quantities. At each step in this epoch, agent \(\ell\) picks arm \(k\) with probability \(q_{k, \ell}^m \coloneqq \frac{n^m_{k, \ell}}{N_{\max}^m}\). Let \(Y_{k, \ell}^t\) be an indicator for arm \(k\) being pulled in step \(t\) by agent \(\ell\). Let \(R_{k, \ell}^t\) be the stochastic reward of arm \(k\) on step \(t\) for agent \(\ell\). and \(c^t_{k, \ell} \coloneqq \tilde{R}_{k, \ell}^t - R_{k, \ell}^t\) be the corruption added to arm \(k\) by the adversary in step \(t\) for agent \(\ell\). Note that \(c^t_{k, \ell}\) may depend on all the stochastic rewards up to (and including) round \(t\), and also on all previous choices of the algorithm (though not the choice at step \(t\). Finally, if we denote \(E^m = \{T^{m-1} + 1, . . . , T^{m}\}\) to be the \(N_{\max}^{m}\) timesteps in epoch \(m\), then we define a random variable \(r_{k}^m\) as follows:
    \begin{equation}
        r_{k}^m = \frac{1}{n_{k}^m}\sum_{\ell \in \mathcal{L}_k}\sum_{t \in E^m}Y_{k, \ell}^t(R_{k, \ell}^t + c_{k, \ell}^t).
    \end{equation}
    Let us break this sum into two:
    \begin{align*}
        A_{k}^m & = \sum_{\ell \in \mathcal{L}_k}\sum_{t \in E^m}Y_{k, \ell}^tR_{k, \ell}^t  \\
        B_{k}^m & = \sum_{\ell \in \mathcal{L}_k}\sum_{t \in E^m}Y_{k, \ell}^tc_{k, \ell}^t.
    \end{align*}

    \item
    \paragraph{Bounding the first and the second part} To \textbf{bound the first part}, we first note that:
    \begin{align*}
        \mathbb{E}\left[A_{k}^m\right] = \sum_{\ell \in \mathcal{L}_k}N^m_{\max}.\left(q_{k, \ell}^m\mu_k\right) = n_{k}^m\mu_k,
    \end{align*}
    Where \(n_{k}^m = \sum_{\ell \in \mathcal{L}_k} \frac{n_{k, \ell}^m}{L_k}\).
    Therefore, according to the Chernoff-Hoeffding bound \cite{dubhashi2009concentration}, for \(\beta \leq 1\) we have:
    \begin{align}
        \label{eqn:A2}
        Pr\left[\left|\frac{A_{k}^m}{n_{k}^m} - \mu_k\right| \geq \sqrt{\frac{3\ln{\frac{4}{\beta}}}{n_{k}^m}}\right] \leq \frac{\beta}{2}.
    \end{align}


    Next, we aim to \textbf{bound the second part}. To this end, we define the sequence of r.v.s, \(\{X_{t, l}\}_{t\in[1,\dots, T], \ell \in \mathcal{L}_ks}\) for agent \(\ell\), where \(X_{t, \ell} = \left(Y_{k, \ell}^t - q_{k, \ell}^m\right)\cdot c_{k, \ell}^t\) for all \(t\). Then \(\{X_{t, l}\}_{t\in[1,\dots, T], \ell \in \mathcal{L}_ks}\) is a martingale sequence with respect to the filtration \(\{\mathcal{F}_t\}_{t=1}^T\) generated by r.v.s \(\{Y_{k, h}^s\}_{h \in \mathcal{L}, k \in \mathcal{K}_h, s \leq t}\) and \(\{R_{k, h}^s\}_{h \in \mathcal{L}, k \in \mathcal{K}_h, s \leq t}\). The corruption \(c_{k, \ell}^m\) becomes deterministic conditioned on \(\mathcal{F}_{t-1}\), and since \(\mathbb{E}\left[Y_{k, \ell}^t | \mathcal{F}_{t-1}\right] = q_{k, \ell}^m\), we have:
    \begin{align*}
        \mathbb{E}\left[X_{t, \ell} | \mathcal{F}_{t-1}\right] = \mathbb{E}\left[Y_{k, \ell}^t - q_{k, \ell}^m | \mathcal{F}_{t-1}\right]\cdot c_{k, \ell}^t = 0.
    \end{align*}

    As \(\left|X_{t, \ell}\right| \leq 1\), using a Freedman-type concentration inequality introduced in \citeauthor{beygelzimer2011contextual}, the predictive quadratic variation of this martingale can be bounded as:
    \begin{gather*}
        \Pr\left[\sum_{\ell \in \mathcal{L}_k}\sum_{t\in E^m} X_{t, \ell} \geq V + \ln \frac{4}{\beta}\right] \leq \frac{\beta}{4},
    \end{gather*}
    where
    \begin{align*}
        V = & \sum_{\ell \in \mathcal{L}_k}\sum_{t \in E^m}\mathbb{E}\left[X_t^2 | \mathcal{F}_{t-1}\right] \leq \sum_{\ell \in \mathcal{L}_k}\sum_{t \in E^m} \left|c_{k, \ell}^t\right|\text{Var}\left(Y_{k, \ell}^t\right) \leq \sum_{\ell \in \mathcal{L}_k}q_{k, \ell}^m\sum_{t \in E^m} \left|c_{k, \ell}^t\right|.
    \end{align*}
    Therefore, we obtain that with a probability of \(1 - \frac{\beta}{4}\):
    \begin{align*}
        \frac{B_{k}^m}{n_{k}^m} & \overset{(a)}\leq \sum_{\ell \in \mathcal{L}_k}\frac{q_{k, \ell}^m}{n_{k}^m}\sum_{t \in E^m} c_{k, \ell}^t + \frac{1}{n_{k}^m} \left(V + \ln{\frac{4}{\beta}}\right) \\
                                & \leq 2\sum_{\ell \in \mathcal{L}_k}\frac{q_{k, \ell}^m}{n_{k}^m}\sum_{t \in E^m} \left|c_{k, \ell}^t\right| + \frac{1}{n_{k}^m} \ln{\frac{4}{\beta}},
    \end{align*}
    where (a) is because \(\sum_{\ell \in \mathcal{L}_k}\sum_{t \in E^m}X_t = \sum_{\ell \in \mathcal{L}_k}\sum_{t \in E^m}(Y_{k, \ell}^t - q_{k, \ell}^m)\cdot c_{k, \ell}^t = B_{k}^m - \sum_{\ell \in \mathcal{L}_k}{q_{k, \ell}^m}\sum_{t \in E^m} c_{k, \ell}^t\).

    We know that \(q_{k, \ell}^m = \frac{n^m_{k, \ell}}{N_{\max}^m}\). We also define the corruption on agent \(\ell\)'s rewards as \(C_{\ell}^m = \sum_{t \in E^m}\max_{k \in \mathcal{K}_{\ell}} |c_{k, \ell}^t|\), therefore we can conclude that \(\sum_{t \in E^m} \left|c_{k, \ell}^t\right| \leq C_{\ell}^m\). We choose a parameter \(\beta \geq 4e^{(-\lambda/16)}\), therefore \(n_{k, \ell}^m \geq \lambda \geq 16\ln{\left(4/\beta\right)}\), and so \(n_{k}^m \geq \lambda \geq 16\ln{\left(4/\beta\right)}\). Then we can rewrite the same bound as:
    \begin{align}
        \label{eqn:B_corr_2}
        \frac{B_{k}^m}{n_{k}^m}\leq 2\sum_{\ell \in \mathcal{L}_k}\frac{n^m_{k, \ell}}{n_k^m}\frac{C^m_\ell}{N^m_{\max}} + \sqrt{\frac{\ln{\frac{4}{\beta}}}{16n_{k}^m}}.
    \end{align}
    \eqref{eqn:B_corr_2} holds for \(-\frac{B_{k}^m}{n_{k, \ell}^m}\) with the same probability, Therefore we have:
    \begin{align}
        \label{eqn:B}
        Pr\left[\left|\frac{B_{k}^m}{n_{k}^m}\right| \leq 2\sum_{\ell \in \mathcal{L}_k}\frac{n^m_{k, \ell}}{n_k^m}\frac{C^m_\ell}{N^m_{\max}} + \sqrt{\frac{\ln{\frac{4}{\beta}}}{16n_{k}^m}}\right] \leq \frac{\beta}{2}.
    \end{align}

    \item
    \paragraph{Combining the two small probability bounds}Combining \eqref{eqn:A2} and \eqref{eqn:B}, we have:
    \begin{align*}
        Pr\left[\left|r_{k}^m - \mu_k\right| \geq 2\sum_{\ell \in \mathcal{L}_k}\frac{n^m_{k, \ell}}{n_k^m}\frac{C^m_\ell}{N^m_{\max}} + \sqrt{4\frac{\ln{\frac{4}{\beta}}}{n_{k}^m}}\right] \leq \beta.
    \end{align*}
    Then we set \(\beta = \delta/(2K\log{T})\), as this value satisfies \(\beta \geq 4e^{-\lambda/16}\), we have:
    \begin{align*}
        Pr\left[\left|r_{k}^m - \mu_k\right| \geq 2\sum_{\ell \in \mathcal{L}_k}\frac{n^m_{k, \ell}}{n_k^m}\frac{C^m_\ell}{N^m_{\max}} + \frac{\Delta_{k, \max}^m}{16}\right] \leq \delta/(2K\log{T}).
    \end{align*}
    \item
    \begin{claim}
        \begin{align}
            \Pr\left[\Tilde{n}_{k, \ell}^m \geq 2 \cdot n_{k, \ell}^m\right] \leq \beta
        \end{align}
    \end{claim}

    \begin{proof}
        Again, we can use a Chernoff-Hoeffding bound on the r.v. representing the actual number of pulls of arm \(k\) by agent \(\ell\) in eopch \(m\), which is: \(\tilde{n}_{k, \ell}^m \coloneqq \sum_{t \in E^m_\ell} Y_{k, \ell}^t\). The expected value of this r.v. is \(\mathbb{E}\left[\tilde{n}_{k, \ell}^m\right] = {n_{k, \ell}^m}\). The probability that the r.v. is more than twice its expectation is at most: \(2\exp{\left(-\frac{n_{k, \ell}^m}{3}\right)} \leq 2\exp{\left(-\frac{\lambda}{3}\right)} \leq 4\exp{\left(\frac{-\lambda}{16}\right)} \leq \beta\).
    \end{proof}

    Therefore using a union bound, we have:
    \begin{align}\label{eq:lem2_1}
        \Pr\bigg[ & \forall k\in \mathcal{K}, m \in \{1, 2, \dots, M\}: \left|r_{k}^m - \mu_k\right| \geq 2\max_{\ell \in \mathcal{L}_k}\frac{C^m_\ell}{N^m_{\max}} + \frac{\Delta_{k, \max}^m}{16} \text{ and } \Tilde{n}_{k, \ell}^m \geq 2 \cdot n_{k, \ell}^m \bigg] \leq \delta.
    \end{align}

\end{proof}

Now let us define \(D^m\) as:
\begin{equation}\label{eq:dm_d_b}
    D^m = 2\max_{\ell \in \mathcal{L}}\frac{C^m_\ell}{N^m_{\max}},
\end{equation}

% \textbf{Lemma 5.}
\begin{lemma}
    Suppose that \(\mathcal{E}\) happens, then for all epochs \(m\):
    \label{lem:5_2}
    \begin{align}
        -D^m - \frac{\Delta^{m - 1}_{k_{*, \ell}, \max}}{8} \leq r_{*, \ell}^m - \mu_{*, \ell} \leq D^m.
    \end{align}
    where
\end{lemma}


\begin{proof}
    We know that \(r_{*, \ell}^m = \max_{k\in\mathcal{K}_\ell}{\{r_{k}^m - \frac{1}{16}\Delta_{k, \max}^{m - 1}\}}\) and therefore \(r_{*, \ell}^m \geq r_{k_{*, \ell}}^m - \frac{1}{16}\Delta_{k_{*, \ell}, \max}^{m - 1}\). Considering the lower bound implied by \(\mathcal{E}\) we have:
    \begin{align*}
        -2\max_{\ell \in \mathcal{L}}\frac{C^m_\ell}{N^m_{\max}} - \frac{\Delta_{k_{*, \ell}, \max}^{m - 1}}{8} \leq r_{*, \ell}^m - \mu_{*, \ell},
    \end{align*}
    since \(\mathcal{L}_{k_{*, \ell}} \subseteq \{\ell\} + \mathcal{N}(\ell)\), we have \(C_{\mathcal{L}_{k_{*, \ell}}} \leq C_{\ell} + C_{\mathcal{N}(\ell)}\), therefore we can rewrite the inequality as:
    \begin{align*}
        -D^m - \frac{\Delta_{k_{*, \ell}, \max}^{m - 1}}{8} \leq r_{*, \ell}^m - \mu_{*, \ell},
    \end{align*}
    We also know that:
    \begin{align*}
        r_{*, \ell}^m & = \max_{k\in\mathcal{K}_\ell}{\{r_{k}^m - \frac{1}{16}\Delta_{k, \max}^{m - 1}\}}                                                                                                   \\
                      & \leq \max_{k\in\mathcal{K}_\ell}\{2\max_{\ell \in \mathcal{L}}\frac{C^m_\ell}{N^m_{\max}} + \frac{1}{16}\Delta_{k, \max}^{m - 1} + \mu_{k} - \frac{1}{16}\Delta_{k, \max}^{m - 1}\} \\
                      & \leq \mu_{*, \ell} + D_\ell^m.
    \end{align*}
    Therefore the lemma is proved.
\end{proof}

Then we define \(\rho^m\) as:
\begin{equation}\label{eq:rho_d_2}
    \rho^m = \sum_{s = 1}^{m}\frac{D^s}{8^{m - s}}.
\end{equation}

\begin{lemma}
    \label{lem:6_2}
    Suppose that \(\mathcal{E}\) happens, then for all epochs \(m\), arm \(k\), and agent \(\ell\):
    \begin{align}
        \Delta_{k, \ell}^m \leq 2(\Delta_{k, \ell} + 2^{-m} + \rho^m).
    \end{align}
\end{lemma}



\begin{proof}
    We prove this by induction on \(m\). For \(m = 1\), the claim is true for all \(k\) and \(\ell\), as \(\Delta_{k, \ell}^m \leq 1 \leq 2\cdot2^{-m}\).

    Suppose that the claim holds for \(m - 1\). Using Lemma~\ref{lem:5_2} and the definition  of the event \(\mathcal{E}\), we write:
    \begin{equation}
        % \resizebox{.94\linewidth}{!}{
        \begin{split}
            \quad r_{*, \ell}^m - r_{k, \ell}^m & = (r_{*, \ell}^m - \mu_{*,\ell}) + (\mu_{*,\ell} - \mu_k) + (\mu_k - r_{k, \ell}^m)                                                                      \\
                                                & \overset{(a)}\leq D^m + \Delta_{k, \ell} + D^m + \frac{\Delta^{m - 1}_{k, \max}}{16}                                                                     \\
                                                & \overset{(b)}\leq \Delta_{k, \ell} + 2D^m + \frac{1}{8}\left(\Delta_{k, \ell} + 2^{-(m-1)} + \sum_{s = 1}^{m-1}\frac{D^{s}_\ell}{8^{(m - 1) - s}}\right) \\
                                                & \leq 2\left(\Delta_{k, \ell} + 2^{-m} + \sum_{s = 1}^{m}\frac{D^{s}_\ell}{8^{m - s}}\right),
        \end{split}
        % }
    \end{equation}
    where inequality (a) holds because \((r_{*, \ell}^m - \mu_{*,\ell})\) is bound using Lemma~\ref{lem:5_2}, and \((\mu_k - r_{k, \ell}^m)\) is bound following the assumption of event \(\mathcal{E}\). Also, inequality (b) holds due to the induction's hypothesis.
    Therefore Lemma~\ref{lem:6_2} is proved.
\end{proof}


\begin{lemma}
    \label{lem:7_2}
    Suppose that \(\mathcal{E}\) happens, then for all epochs \(m\), arm \(k\), and agent \(\ell\):
    \begin{align}
        \Delta_{k, \ell}^m \geq \frac{1}{2} \Delta_{k, \ell} - 3\rho^m -\frac{3}{4}2^{-m}.
    \end{align}
\end{lemma}

\begin{proof}
    \begin{align*}
        \Delta_{k, \ell}^m  \geq r_{*, \ell}^m - r_{k, \ell}^m
         & \overset{(a)}\geq \left(\mu_{*, \ell} - D^m - \frac{\Delta^{m - 1}_{k_{*, \ell}, \max}}{8}\right) - \left(\mu_k + D^m + \frac{\Delta^{m - 1}_{k, \max}}{16}\right) \\
         & \overset{(b)}\geq \Delta_{k, \ell} - 2D^m - \left(\frac{3}{8}\rho^{m-1} + \frac{3}{8}2^{-(m - 1)} + \frac{3}{8}\Delta_{k, \ell}\right)                             \\
         & \geq \frac{1}{2} \Delta_{k, \ell} - 3\sum_{s = 1}^{m}\frac{D_{\ell}^{s}}{8^{m - s}} -\frac{3}{4}2^{-m}.
    \end{align*}
    where (a) holds because \(r_{*, \ell}^m\) can be bound using Lemma~\ref{lem:5_2}, and \(r_{k, \ell}^m\) is bound due to event \(\mathcal{E}\), and (b) is because of Lemma~\ref{lem:6_2}.
\end{proof}



\subsection{\distbarbar Homogeneous case}\label{appendix:b_1_2}
In the homogeneous case, all agents have access to all arms. Therefore, at every epoch, \(r_{*, \ell_1}^m = r_{*, \ell_2}^m\) for every agent pair \(\ell_1\) and \(\ell_2\). Consequently, \(\Delta_{k, \ell_1}^m = \Delta_{k, \ell_2}^m\) and thus \(n_{k, \ell_1}^m = n_{k, \ell_2}^m\).

We can then rewrite \eqref{eq:lem2_1} and redefine the event \(\mathcal{E}\) as:
\begin{align}\label{eq:event-E_d_2_h}
    \mathcal{E} \coloneqq \left\{\forall k\in \mathcal{K}, \ell\in \mathcal{L}, m \in \{1, 2, \dots, M\} : \left|r_{k}^m - \mu_k\right| \geq \frac{2}{L}\sum_{\ell \in \mathcal{L}}\frac{C^m_\ell}{N^m_{\max}} + \frac{\Delta_{k, \max}^{m-1}}{16} \text{ and } \Tilde{n}_{k, \ell}^m \geq {2 n_{k, \ell}^m} \right\},
\end{align}

Subsequently, we define \(D^m\) as:
\begin{equation}\label{eq:dm_d_b_2}
    D^m = \frac{2}{L}\sum_{\ell \in \mathcal{L}}\frac{C^m_\ell}{N^m_{\max}}.
\end{equation}
Following the same proof as in Appendix~\ref{appendix:a_1}, we can upper bound the total regret as:
\begin{align}
    O\left(KC + \log{\left(\frac{K}{\delta}\log{T}\right)}\sum_{k \in \mathcal{K}}\frac{\sum_{\ell \in \mathcal{L}_k}\left(\Delta_{k, \ell}\right)^{-1}}{L_{k}}\log{T}\right).
\end{align}


\subsection{\distbarbar Tightness (Proof for Theorem~\ref{theo:4})}\label{appendix:b_2}
% \subsubsection{Proof for Theorem~\ref{theo:4}}

\begin{proof}
    Here we aim to give an example here that suffers the regret of \(\Omega\left(\sum_{\ell \in \mathcal{L}} \sum_{k \in \mathcal{K}_\ell} \frac{\hat L}{L_k}\max_{\ell \in \mathcal{L}_k}C_{\ell}\right)\). Consider the case where every arm is accessible by exactly \(L'\) agents. Among these arms only one has a expected reward of 1, let us call that arm 1. And others have an expected reward equal to 0.

    In the case without corruption, for each epoch \(m \geq 1\) and for any agent \(\ell \in \mathcal{L}_1\), we have \(\Delta^m_{1, \ell} = 2^{-m}\), as \(\Delta^m_{1, \ell} = \max{\{2^{-m}, r_{*, \ell}^m - r_{1}^m\}}\), and \(r_{*, \ell}^m = r_{1}^m\). And, for every other \(k \in \mathcal{K}_\ell\), \(\Delta_{k, \ell}^m = r^m_{*, \ell} = {1} - \frac{(1) - (1/16)^m}{15} \in [14/15, 15/16]\).
    Therefore, with no corruption, the \(m\)th epoch has length:
    \begin{align*}
        N^m_\ell = \frac{\lambda}{L'}\left(2^{2(m-1)}+O\left(K_\ell\right)\right).
    \end{align*}


    Now consider a case where the rewards of arm 1 is corrupted in every round of a certain epoch \(m\in\{1,2,\dots,M\}\). Therefore the total amount of corruption is equal to:
    \begin{align*}
        C = \sum_{\ell \in \mathcal{L}_1} C_\ell = \sum_{\ell \in \mathcal{L}_1} \frac{\lambda}{L'}\left(2^{2(m - 1)}+O\left(K_\ell\right)\right)= \lambda\left(2^{2(m - 1)}+ \sum_{\ell \in \mathcal{L}_1}O\left(K_\ell\right)\right).
    \end{align*}

    Note that the corruption is only affecting arm \(1\), making every observed reward equal to \(0\). Therefore \(r^m_{*, \ell} \leq 0\) and all \(\Delta_{k, \ell}^m = 2^{-m}\). And therefore the length of the next epoch for agent \(\ell \in \mathcal{L}_1\) will be:
    \begin{align*}
        N^{m+1}_\ell = \lambda2^{2m}\sum_{k \in \mathcal{K}_\ell}\frac{1}{L'} = \Omega\left(\frac{CK_\ell}{L'}\right).
    \end{align*}

    Therefore in epoch \(m+1\), agent \(\ell \in \mathcal{L}_1\) has \(\frac{C(K_\ell - 1)}{L'}\) arm pulls with reward \(0\), which causes a total regret of \(O\left(L' \times \frac{CK}{L'}\right)\). As in this case, \(\hat L\) and \(L_k\) are equal to \(L'\) for all \(k \in \mathcal{K}\), and \(\max_{\ell \in \mathcal{L}_k}C_{\ell} = \frac{C}{L'}\), therefore \(\Omega\left(\sum_{\ell \in \mathcal{L}} \sum_{k \in \mathcal{K}_\ell} \frac{\hat L}{L_k}\max_{\ell \in \mathcal{L}_k}C_{\ell}\right) = \Omega\left(KC\right)\).

\end{proof}
